# Supplementary material for: TimePoint: Accelerated Time Series Alignment via Self-Supervised Keypoint and Descriptor Learning
Source: arXiv:2505.23475 source file (2025-05-29)
Supplement: Supplementary file 1 [file all_ucr_tp10.pdf]

| TP | Dataset | Keypoints Percentage | Accuracy | F1 Score | Precision | Recall |
|---|---|---|---|---|---|---|
| TP + Dense | SmoothSubspace | 0.1 | 0.8 | 0.8 | 0.8 | 0.8 |
| TP + Dense | Chinatown | 0.1 | 0.898 | 0.863 | 0.903 | 0.879 |
| TP + Dense | ItalyPowerDemand | 0.1 | 0.892 | 0.893 | 0.892 | 0.892 |
| TP + Dense | MelbournePedestrian | 0.1 | 0.1 | 0.01 | 0.1 | 0.018 |
| TP + Dense | Crop | 0.1 | 0.659 | 0.64 | 0.659 | 0.647 |
| TP + Dense | SyntheticControl | 0.1 | 0.96 | 0.962 | 0.96 | 0.96 |
| TP + Dense | SonyAIBORobotSurface2 | 0.1 | 0.829 | 0.821 | 0.837 | 0.824 |
| TP + Dense | SonyAIBORobotSurface1 | 0.1 | 0.699 | 0.794 | 0.736 | 0.691 |
| TP + Dense | DistalPhalanxOutlineAgeGroup | 0.1 | 0.669 | 0.616 | 0.665 | 0.629 |
| TP + Dense | DistalPhalanxOutlineCorrect | 0.1 | 0.732 | 0.729 | 0.711 | 0.715 |
| TP + Dense | DistalPhalanxTW | 0.1 | 0.597 | 0.437 | 0.443 | 0.436 |
| TP + Dense | MiddlePhalanxOutlineAgeGroup | 0.1 | 0.442 | 0.394 | 0.4 | 0.393 |
| TP + Dense | MiddlePhalanxOutlineCorrect | 0.1 | 0.656 | 0.657 | 0.66 | 0.655 |
| TP + Dense | MiddlePhalanxTW | 0.1 | 0.448 | 0.362 | 0.349 | 0.349 |
| TP + Dense | PhalangesOutlinesCorrect | 0.1 | 0.719 | 0.703 | 0.695 | 0.698 |
| TP + Dense | ProximalPhalanxOutlineAgeGroup | 0.1 | 0.761 | 0.65 | 0.675 | 0.653 |
| TP + Dense | ProximalPhalanxOutlineCorrect | 0.1 | 0.784 | 0.764 | 0.707 | 0.723 |
| TP + Dense | ProximalPhalanxTW | 0.1 | 0.722 | 0.437 | 0.414 | 0.415 |
| TP + Dense | TwoLeadECG | 0.1 | 0.851 | 0.852 | 0.851 | 0.851 |
| TP + Dense | MoteStrain | 0.1 | 0.819 | 0.826 | 0.812 | 0.815 |
| TP + Dense | ECG200 | 0.1 | 0.82 | 0.81 | 0.793 | 0.799 |
| TP + Dense | ElectricDevices | 0.1 | 0.592 | 0.533 | 0.487 | 0.5 |
| TP + Dense | MedicalImages | 0.1 | 0.707 | 0.693 | 0.671 | 0.675 |

| | | | | | | |
|---|---|---|---|---|---|---|
| TP + Dense | BME | 0.1 | 0.92 | 0.935 | 0.92 | 0.92 |
| TP + Dense | CBF | 0.1 | 0.97 | 0.971 | 0.97 | 0.97 |
| TP + Dense | SwedishLeaf | 0.1 | 0.877 | 0.884 | 0.879 | 0.879 |
| TP + Dense | TwoPatterns | 0.1 | 0.963 | 0.963 | 0.963 | 0.963 |
| TP + Dense | FaceAll | 0.1 | 0.691 | 0.747 | 0.785 | 0.716 |
| TP + Dense | FacesUCR | 0.1 | 0.84 | 0.841 | 0.808 | 0.816 |
| TP + Dense | ECGFiveDays | 0.1 | 0.693 | 0.727 | 0.694 | 0.682 |

| TP | Dataset | Keypoints Percentage | Accuracy | F1 Score | Precision | Recall |
|---|---|---|---|---|---|---|
| TP + Dense | ECG5000 | 0.1 | 0.927 | 0.643 | 0.552 | 0.576 |
| TP + Dense | Plane | 0.1 | 1.0 | 1.0 | 1.0 | 1.0 |
| TP + Dense | PowerCons | 0.1 | 0.906 | 0.906 | 0.906 | 0.906 |
| TP + Dense | GunPoint | 0.1 | 0.96 | 0.962 | 0.961 | 0.96 |
| TP + Dense | GunPointAgeSpan | 0.1 | 0.975 | 0.975 | 0.975 | 0.975 |
| TP + Dense | GunPointMaleVersusFemale | 0.1 | 0.997 | 0.997 | 0.997 | 0.997 |
| TP + Dense | GunPointOldVersusYoung | 0.1 | 0.946 | 0.951 | 0.944 | 0.946 |
| TP + Dense | UMD | 0.1 | 0.951 | 0.955 | 0.951 | 0.951 |
| TP + Dense | Wafer | 0.1 | 0.977 | 0.973 | 0.904 | 0.935 |
| TP + Dense | ChlorineConcentration | 0.1 | 0.584 | 0.539 | 0.535 | 0.537 |
| TP + Dense | Adiac | 0.1 | 0.471 | 0.494 | 0.473 | 0.464 |
| TP + Dense | Fungi | 0.1 | 0.866 | 0.888 | 0.902 | 0.883 |
| TP + Dense | Wine | 0.1 | 0.667 | 0.668 | 0.667 | 0.666 |
| TP + Dense | Strawberry | 0.1 | 0.941 | 0.931 | 0.944 | 0.936 |
| TP + Dense | ArrowHead | 0.1 | 0.766 | 0.789 | 0.782 | 0.767 |

| | | | | | | |
|---|---|---|---|---|---|---|
| TP + Dense | InsectWingbeatSound | 0.1 | 0.37 | 0.366 | 0.37 | 0.364 |
| TP + Dense | FiftyWords | 0.1 | 0.723 | 0.619 | 0.613 | 0.589 |
| TP + Dense | WordSynonyms | 0.1 | 0.705 | 0.661 | 0.587 | 0.599 |
| TP + Dense | Trace | 0.1 | 1.0 | 1.0 | 1.0 | 1.0 |
| TP + Dense | ToeSegmentation1 | 0.1 | 0.877 | 0.892 | 0.872 | 0.875 |
| TP + Dense | Coffee | 0.1 | 1.0 | 1.0 | 1.0 | 1.0 |
| TP + Dense | DodgerLoopDay | 0.1 | 0.15 | 0.021 | 0.143 | 0.037 |
| TP + Dense | DodgerLoopGame | 0.1 | 0.478 | 0.239 | 0.5 | 0.324 |
| TP + Dense | DodgerLoopWeekend | 0.1 | 0.261 | 0.13 | 0.5 | 0.207 |
| TP + Dense | CricketX | 0.1 | 0.767 | 0.773 | 0.772 | 0.768 |
| TP + Dense | CricketY | 0.1 | 0.733 | 0.752 | 0.735 | 0.741 |
| TP + Dense | CricketZ | 0.1 | 0.8 | 0.797 | 0.794 | 0.792 |
| TP + Dense | FreezerRegularTrain | 0.1 | 0.919 | 0.919 | 0.919 | 0.919 |
| TP + Dense | FreezerSmallTrain | 0.1 | 0.801 | 0.802 | 0.801 | 0.801 |
| TP + Dense | UWaveGestureLibraryX | 0.1 | 0.773 | 0.755 | 0.77 | 0.758 |

| TP | Dataset | Keypoints Percentage | Accuracy | F1 Score | Precision | Recall |
|---|---|---|---|---|---|---|
| TP + Dense | UWaveGestureLibraryY | 0.1 | 0.67 | 0.668 | 0.671 | 0.664 |
| TP + Dense | UWaveGestureLibraryZ | 0.1 | 0.688 | 0.675 | 0.689 | 0.673 |
| TP + Dense | Lightning7 | 0.1 | 0.699 | 0.72 | 0.704 | 0.699 |
| TP + Dense | ToeSegmentation2 | 0.1 | 0.892 | 0.817 | 0.837 | 0.827 |
| TP + Dense | DiatomSizeReduction | 0.1 | 0.928 | 0.947 | 0.902 | 0.918 |
| TP + Dense | FaceFour | 0.1 | 0.852 | 0.88 | 0.872 | 0.857 |
| TP + Dense | GestureMidAirD1 | 0.1 | 0.038 | 0.001 | 0.038 | 0.003 |

| | | | | | | |
|---|---|---|---|---|---|---|
| TP + Dense | GestureMidAirD2 | 0.1 | 0.038 | 0.001 | 0.038 | 0.003 |
| TP + Dense | GestureMidAirD3 | 0.1 | 0.038 | 0.001 | 0.038 | 0.003 |
| TP + Dense | PickupGestureWiimoteZ | 0.1 | 0.1 | 0.01 | 0.1 | 0.018 |
| TP + Dense | AllGestureWiimoteX | 0.1 | 0.1 | 0.01 | 0.1 | 0.018 |
| TP + Dense | AllGestureWiimoteY | 0.1 | 0.1 | 0.01 | 0.1 | 0.018 |
| TP + Dense | AllGestureWiimoteZ | 0.1 | 0.1 | 0.01 | 0.1 | 0.018 |
| TP + Dense | ShakeGestureWiimoteZ | 0.1 | 0.1 | 0.01 | 0.1 | 0.018 |
| TP + Dense | Symbols | 0.1 | 0.934 | 0.944 | 0.931 | 0.932 |
| TP + Dense | Yoga | 0.1 | 0.816 | 0.82 | 0.81 | 0.812 |
| TP + Dense | OSULeaf | 0.1 | 0.727 | 0.758 | 0.732 | 0.738 |
| TP + Dense | Ham | 0.1 | 0.59 | 0.592 | 0.592 | 0.59 |
| TP + Dense | Meat | 0.1 | 0.883 | 0.892 | 0.883 | 0.885 |
| TP + Dense | GesturePebbleZ1 | 0.1 | 0.163 | 0.027 | 0.167 | 0.047 |
| TP + Dense | GesturePebbleZ2 | 0.1 | 0.152 | 0.025 | 0.167 | 0.044 |
| TP + Dense | Fish | 0.1 | 0.76 | 0.787 | 0.76 | 0.752 |
| TP + Dense | Beef | 0.1 | 0.633 | 0.737 | 0.633 | 0.635 |
| TP + Dense | FordA | 0.1 | 0.779 | 0.78 | 0.777 | 0.778 |
| TP + Dense | FordB | 0.1 | 0.694 | 0.694 | 0.694 | 0.693 |
| TP + Dense | ShapeletSim | 0.1 | 0.556 | 0.557 | 0.556 | 0.552 |
| TP + Dense | BeetleFly | 0.1 | 0.75 | 0.833 | 0.75 | 0.733 |
| TP + Dense | BirdChicken | 0.1 | 0.65 | 0.652 | 0.65 | 0.649 |
| TP + Dense | Earthquakes | 0.1 | 0.683 | 0.551 | 0.542 | 0.543 |
| TP + Dense | Herring | 0.1 | 0.469 | 0.48 | 0.48 | 0.468 |

| TP | Dataset | Keypoints Percentage | Accuracy | F1 Score | Precision | Recall |
|---|---|---|---|---|---|---|
| TP + Dense | ShapesAll | 0.1 | 0.837 | 0.852 | 0.837 | 0.831 |
| TP + Dense | OliveOil | 0.1 | 0.767 | 0.799 | 0.669 | 0.7 |
| TP + Dense | Car | 0.1 | 0.767 | 0.758 | 0.764 | 0.753 |
| TP + Dense | InsectEPGRegularTrain | 0.1 | 0.936 | 0.944 | 0.909 | 0.924 |
| TP + Dense | InsectEPGSmallTrain | 0.1 | 0.843 | 0.822 | 0.861 | 0.83 |
| TP + Dense | Lightning2 | 0.1 | 0.803 | 0.806 | 0.807 | 0.803 |
| TP + Dense | Computers | 0.1 | 0.616 | 0.617 | 0.616 | 0.615 |
| TP + Dense | LargeKitchenAppliances | 0.1 | 0.765 | 0.77 | 0.765 | 0.763 |
| TP + Dense | RefrigerationDevices | 0.1 | 0.469 | 0.478 | 0.469 | 0.472 |
| TP + Dense | ScreenType | 0.1 | 0.448 | 0.456 | 0.448 | 0.448 |
| TP + Dense | SmallKitchenAppliances | 0.1 | 0.608 | 0.617 | 0.608 | 0.608 |
| TP + Dense | NonInvasiveFetalECGThorax1 | 0.1 | 0.734 | 0.76 | 0.732 | 0.725 |
| TP + Dense | NonInvasiveFetalECGThorax2 | 0.1 | 0.803 | 0.804 | 0.797 | 0.795 |
| TP + Dense | Worms | 0.1 | 0.623 | 0.62 | 0.595 | 0.597 |
| TP + Dense | WormsTwoClass | 0.1 | 0.74 | 0.735 | 0.735 | 0.735 |
| TP + WTConv | SmoothSubspace | 0.1 | 0.8 | 0.824 | 0.8 | 0.798 |
| TP + WTConv | Chinatown | 0.1 | 0.831 | 0.787 | 0.814 | 0.798 |
| TP + WTConv | ItalyPowerDemand | 0.1 | 0.941 | 0.941 | 0.941 | 0.941 |
| TP + WTConv | MelbournePedestrian | 0.1 | 0.1 | 0.01 | 0.1 | 0.018 |
| TP + WTConv | Crop | 0.1 | 0.665 | 0.648 | 0.665 | 0.654 |
| TP + WTConv | SyntheticControl | 0.1 | 0.957 | 0.958 | 0.957 | 0.957 |
| TP + WTConv | SonyAIBORobotSurface2 | 0.1 | 0.86 | 0.862 | 0.84 | 0.848 |
| TP + WTConv | SonyAIBORobotSurface1 | 0.1 | 0.839 | 0.856 | 0.856 | 0.839 |

| | | | | | | |
|---|---|---|---|---|---|---|
| TP + WTConv | DistalPhalanxOutlineAgeGroup | 0.1 | 0.583 | 0.512 | 0.532 | 0.515 |
| TP + WTConv | DistalPhalanxOutlineCorrect | 0.1 | 0.652 | 0.64 | 0.635 | 0.636 |
| TP + WTConv | DistalPhalanxTW | 0.1 | 0.511 | 0.382 | 0.388 | 0.379 |
| TP + WTConv | MiddlePhalanxOutlineAgeGroup | 0.1 | 0.422 | 0.351 | 0.35 | 0.349 |
| TP + WTConv | MiddlePhalanxOutlineCorrect | 0.1 | 0.663 | 0.656 | 0.653 | 0.654 |
| TP + WTConv | MiddlePhalanxTW | 0.1 | 0.442 | 0.349 | 0.353 | 0.35 |
| TP + WTConv | PhalangesOutlinesCorrect | 0.1 | 0.69 | 0.673 | 0.672 | 0.673 |

| TP | Dataset | Keypoints Percentage | Accuracy | F1 Score | Precision | Recall |
|---|---|---|---|---|---|---|
| TP + WTConv | ProximalPhalanxOutlineAgeGroup | 0.1 | 0.79 | 0.663 | 0.667 | 0.665 |
| TP + WTConv | ProximalPhalanxOutlineCorrect | 0.1 | 0.818 | 0.812 | 0.75 | 0.769 |
| TP + WTConv | ProximalPhalanxTW | 0.1 | 0.673 | 0.401 | 0.476 | 0.412 |
| TP + WTConv | TwoLeadECG | 0.1 | 0.83 | 0.832 | 0.83 | 0.829 |
| TP + WTConv | MoteStrain | 0.1 | 0.826 | 0.827 | 0.822 | 0.824 |
| TP + WTConv | ECG200 | 0.1 | 0.85 | 0.854 | 0.816 | 0.829 |
| TP + WTConv | ElectricDevices | 0.1 | 0.593 | 0.53 | 0.493 | 0.501 |
| TP + WTConv | MedicalImages | 0.1 | 0.687 | 0.648 | 0.64 | 0.636 |
| TP + WTConv | BME | 0.1 | 0.96 | 0.964 | 0.96 | 0.96 |
| TP + WTConv | CBF | 0.1 | 0.94 | 0.942 | 0.94 | 0.94 |
| TP + WTConv | SwedishLeaf | 0.1 | 0.875 | 0.883 | 0.879 | 0.877 |
| TP + WTConv | TwoPatterns | 0.1 | 0.729 | 0.729 | 0.729 | 0.729 |
| TP + WTConv | FaceAll | 0.1 | 0.676 | 0.704 | 0.765 | 0.676 |
| TP + WTConv | FacesUCR | 0.1 | 0.735 | 0.74 | 0.694 | 0.703 |
| TP + WTConv | ECGFiveDays | 0.1 | 0.812 | 0.823 | 0.812 | 0.81 |

| | | | | | | |
|---|---|---|---|---|---|---|
| TP + WTConv | ECG5000 | 0.1 | 0.921 | 0.711 | 0.567 | 0.593 |
| TP + WTConv | Plane | 0.1 | 1.0 | 1.0 | 1.0 | 1.0 |
| TP + WTConv | PowerCons | 0.1 | 0.856 | 0.864 | 0.856 | 0.855 |
| TP + WTConv | GunPoint | 0.1 | 0.973 | 0.973 | 0.973 | 0.973 |
| TP + WTConv | GunPointAgeSpan | 0.1 | 0.981 | 0.981 | 0.981 | 0.981 |
| TP + WTConv | GunPointMaleVersusFemale | 0.1 | 0.994 | 0.994 | 0.994 | 0.994 |
| TP + WTConv | GunPointOldVersusYoung | 0.1 | 0.968 | 0.971 | 0.967 | 0.968 |
| TP + WTConv | UMD | 0.1 | 0.91 | 0.913 | 0.91 | 0.908 |
| TP + WTConv | Wafer | 0.1 | 0.994 | 0.987 | 0.983 | 0.985 |
| TP + WTConv | ChlorineConcentration | 0.1 | 0.574 | 0.525 | 0.528 | 0.526 |
| TP + WTConv | Adiac | 0.1 | 0.645 | 0.656 | 0.644 | 0.633 |
| TP + WTConv | Fungi | 0.1 | 0.957 | 0.964 | 0.959 | 0.955 |
| TP + WTConv | Wine | 0.1 | 0.611 | 0.612 | 0.611 | 0.61 |
| TP + WTConv | Strawberry | 0.1 | 0.932 | 0.921 | 0.939 | 0.928 |
| TP + WTConv | ArrowHead | 0.1 | 0.869 | 0.867 | 0.871 | 0.868 |

| TP | Dataset | Keypoints Percentage | Accuracy | F1 Score | Precision | Recall |
|---|---|---|---|---|---|---|
| TP + WTConv | InsectWingbeatSound | 0.1 | 0.468 | 0.469 | 0.468 | 0.466 |
| TP + WTConv | FiftyWords | 0.1 | 0.745 | 0.625 | 0.608 | 0.59 |
| TP + WTConv | WordSynonyms | 0.1 | 0.688 | 0.608 | 0.543 | 0.54 |
| TP + WTConv | Trace | 0.1 | 0.99 | 0.988 | 0.991 | 0.989 |
| TP + WTConv | ToeSegmentation1 | 0.1 | 0.846 | 0.849 | 0.849 | 0.846 |
| TP + WTConv | Coffee | 0.1 | 1.0 | 1.0 | 1.0 | 1.0 |
| TP + WTConv | DodgerLoopDay | 0.1 | 0.15 | 0.021 | 0.143 | 0.037 |

| | | | | | | |
|---|---|---|---|---|---|---|
| TP + WTConv | DodgerLoopGame | 0.1 | 0.478 | 0.239 | 0.5 | 0.324 |
| TP + WTConv | DodgerLoopWeekend | 0.1 | 0.261 | 0.13 | 0.5 | 0.207 |
| TP + WTConv | CricketX | 0.1 | 0.715 | 0.733 | 0.724 | 0.718 |
| TP + WTConv | CricketY | 0.1 | 0.664 | 0.677 | 0.664 | 0.667 |
| TP + WTConv | CricketZ | 0.1 | 0.726 | 0.727 | 0.718 | 0.718 |
| TP + WTConv | FreezerRegularTrain | 0.1 | 0.913 | 0.913 | 0.913 | 0.913 |
| TP + WTConv | FreezerSmallTrain | 0.1 | 0.78 | 0.781 | 0.78 | 0.779 |
| TP + WTConv | UWaveGestureLibraryX | 0.1 | 0.758 | 0.745 | 0.756 | 0.748 |
| TP + WTConv | UWaveGestureLibraryY | 0.1 | 0.703 | 0.697 | 0.703 | 0.697 |
| TP + WTConv | UWaveGestureLibraryZ | 0.1 | 0.689 | 0.674 | 0.691 | 0.675 |
| TP + WTConv | Lightning7 | 0.1 | 0.671 | 0.693 | 0.694 | 0.675 |
| TP + WTConv | ToeSegmentation2 | 0.1 | 0.823 | 0.721 | 0.779 | 0.742 |
| TP + WTConv | DiatomSizeReduction | 0.1 | 0.967 | 0.974 | 0.934 | 0.95 |
| TP + WTConv | FaceFour | 0.1 | 0.807 | 0.829 | 0.831 | 0.803 |
| TP + WTConv | GestureMidAirD1 | 0.1 | 0.038 | 0.001 | 0.038 | 0.003 |
| TP + WTConv | GestureMidAirD2 | 0.1 | 0.038 | 0.001 | 0.038 | 0.003 |
| TP + WTConv | GestureMidAirD3 | 0.1 | 0.038 | 0.001 | 0.038 | 0.003 |
| TP + WTConv | PickupGestureWiimoteZ | 0.1 | 0.1 | 0.01 | 0.1 | 0.018 |
| TP + WTConv | AllGestureWiimoteX | 0.1 | 0.1 | 0.01 | 0.1 | 0.018 |
| TP + WTConv | AllGestureWiimoteY | 0.1 | 0.1 | 0.01 | 0.1 | 0.018 |
| TP + WTConv | AllGestureWiimoteZ | 0.1 | 0.1 | 0.01 | 0.1 | 0.018 |
| TP + WTConv | ShakeGestureWiimoteZ | 0.1 | 0.1 | 0.01 | 0.1 | 0.018 |
| TP + WTConv | Symbols | 0.1 | 0.949 | 0.955 | 0.947 | 0.948 |

| TP | Dataset | Keypoints Percentage | Accuracy | F1 Score | Precision | Recall |
|---|---|---|---|---|---|---|
| TP + WTConv | Yoga | 0.1 | 0.858 | 0.86 | 0.854 | 0.856 |
| TP + WTConv | OSULeaf | 0.1 | 0.789 | 0.812 | 0.794 | 0.786 |
| TP + WTConv | Ham | 0.1 | 0.514 | 0.515 | 0.515 | 0.514 |
| TP + WTConv | Meat | 0.1 | 0.9 | 0.905 | 0.9 | 0.901 |
| TP + WTConv | GesturePebbleZ1 | 0.1 | 0.163 | 0.027 | 0.167 | 0.047 |
| TP + WTConv | GesturePebbleZ2 | 0.1 | 0.152 | 0.025 | 0.167 | 0.044 |
| TP + WTConv | Fish | 0.1 | 0.874 | 0.871 | 0.877 | 0.872 |
| TP + WTConv | Beef | 0.1 | 0.733 | 0.773 | 0.733 | 0.741 |
| TP + WTConv | FordA | 0.1 | 0.78 | 0.799 | 0.775 | 0.774 |
| TP + WTConv | FordB | 0.1 | 0.641 | 0.654 | 0.642 | 0.634 |
| TP + WTConv | ShapeletSim | 0.1 | 0.6 | 0.602 | 0.6 | 0.598 |
| TP + WTConv | BeetleFly | 0.1 | 0.95 | 0.955 | 0.95 | 0.95 |
| TP + WTConv | BirdChicken | 0.1 | 0.9 | 0.917 | 0.9 | 0.899 |
| TP + WTConv | Earthquakes | 0.1 | 0.669 | 0.517 | 0.513 | 0.511 |
| TP + WTConv | Herring | 0.1 | 0.469 | 0.449 | 0.449 | 0.449 |
| TP + WTConv | ShapesAll | 0.1 | 0.86 | 0.876 | 0.86 | 0.856 |
| TP + WTConv | OliveOil | 0.1 | 0.567 | 0.523 | 0.489 | 0.493 |
| TP + WTConv | Car | 0.1 | 0.85 | 0.85 | 0.843 | 0.846 |
| TP + WTConv | InsectEPGRegularTrain | 0.1 | 0.964 | 0.966 | 0.951 | 0.958 |
| TP + WTConv | InsectEPGSmallTrain | 0.1 | 0.815 | 0.783 | 0.8 | 0.789 |
| TP + WTConv | Lightning2 | 0.1 | 0.836 | 0.843 | 0.83 | 0.832 |
| TP + WTConv | Computers | 0.1 | 0.668 | 0.668 | 0.668 | 0.668 |
| TP + WTConv | LargeKitchenAppliances | 0.1 | 0.757 | 0.757 | 0.757 | 0.756 |

| | | | | | | |
|---|---|---|---|---|---|---|
| TP + WTConv | RefrigerationDevices | 0.1 | 0.525 | 0.528 | 0.525 | 0.526 |
| TP + WTConv | ScreenType | 0.1 | 0.413 | 0.413 | 0.413 | 0.412 |
| TP + WTConv | SmallKitchenAppliances | 0.1 | 0.555 | 0.562 | 0.555 | 0.55 |
| TP + WTConv | NonInvasiveFetalECGThorax1 | 0.1 | 0.814 | 0.828 | 0.813 | 0.808 |
| TP + WTConv | NonInvasiveFetalECGThorax2 | 0.1 | 0.847 | 0.846 | 0.842 | 0.842 |
| TP + WTConv | Worms | 0.1 | 0.662 | 0.718 | 0.599 | 0.625 |
| TP + WTConv | WormsTwoClass | 0.1 | 0.727 | 0.742 | 0.742 | 0.727 |
