# Supplementary material for: TimePoint: Accelerated Time Series Alignment via Self-Supervised Keypoint and Descriptor Learning
Source: arXiv:2505.23475 source file (2025-05-29)
Supplement: Supplementary file 2 [file fig_supmat_dtw_path.tex]

\begin{figure}
    \centering
    \includegraphics[width=0.49\linewidth]{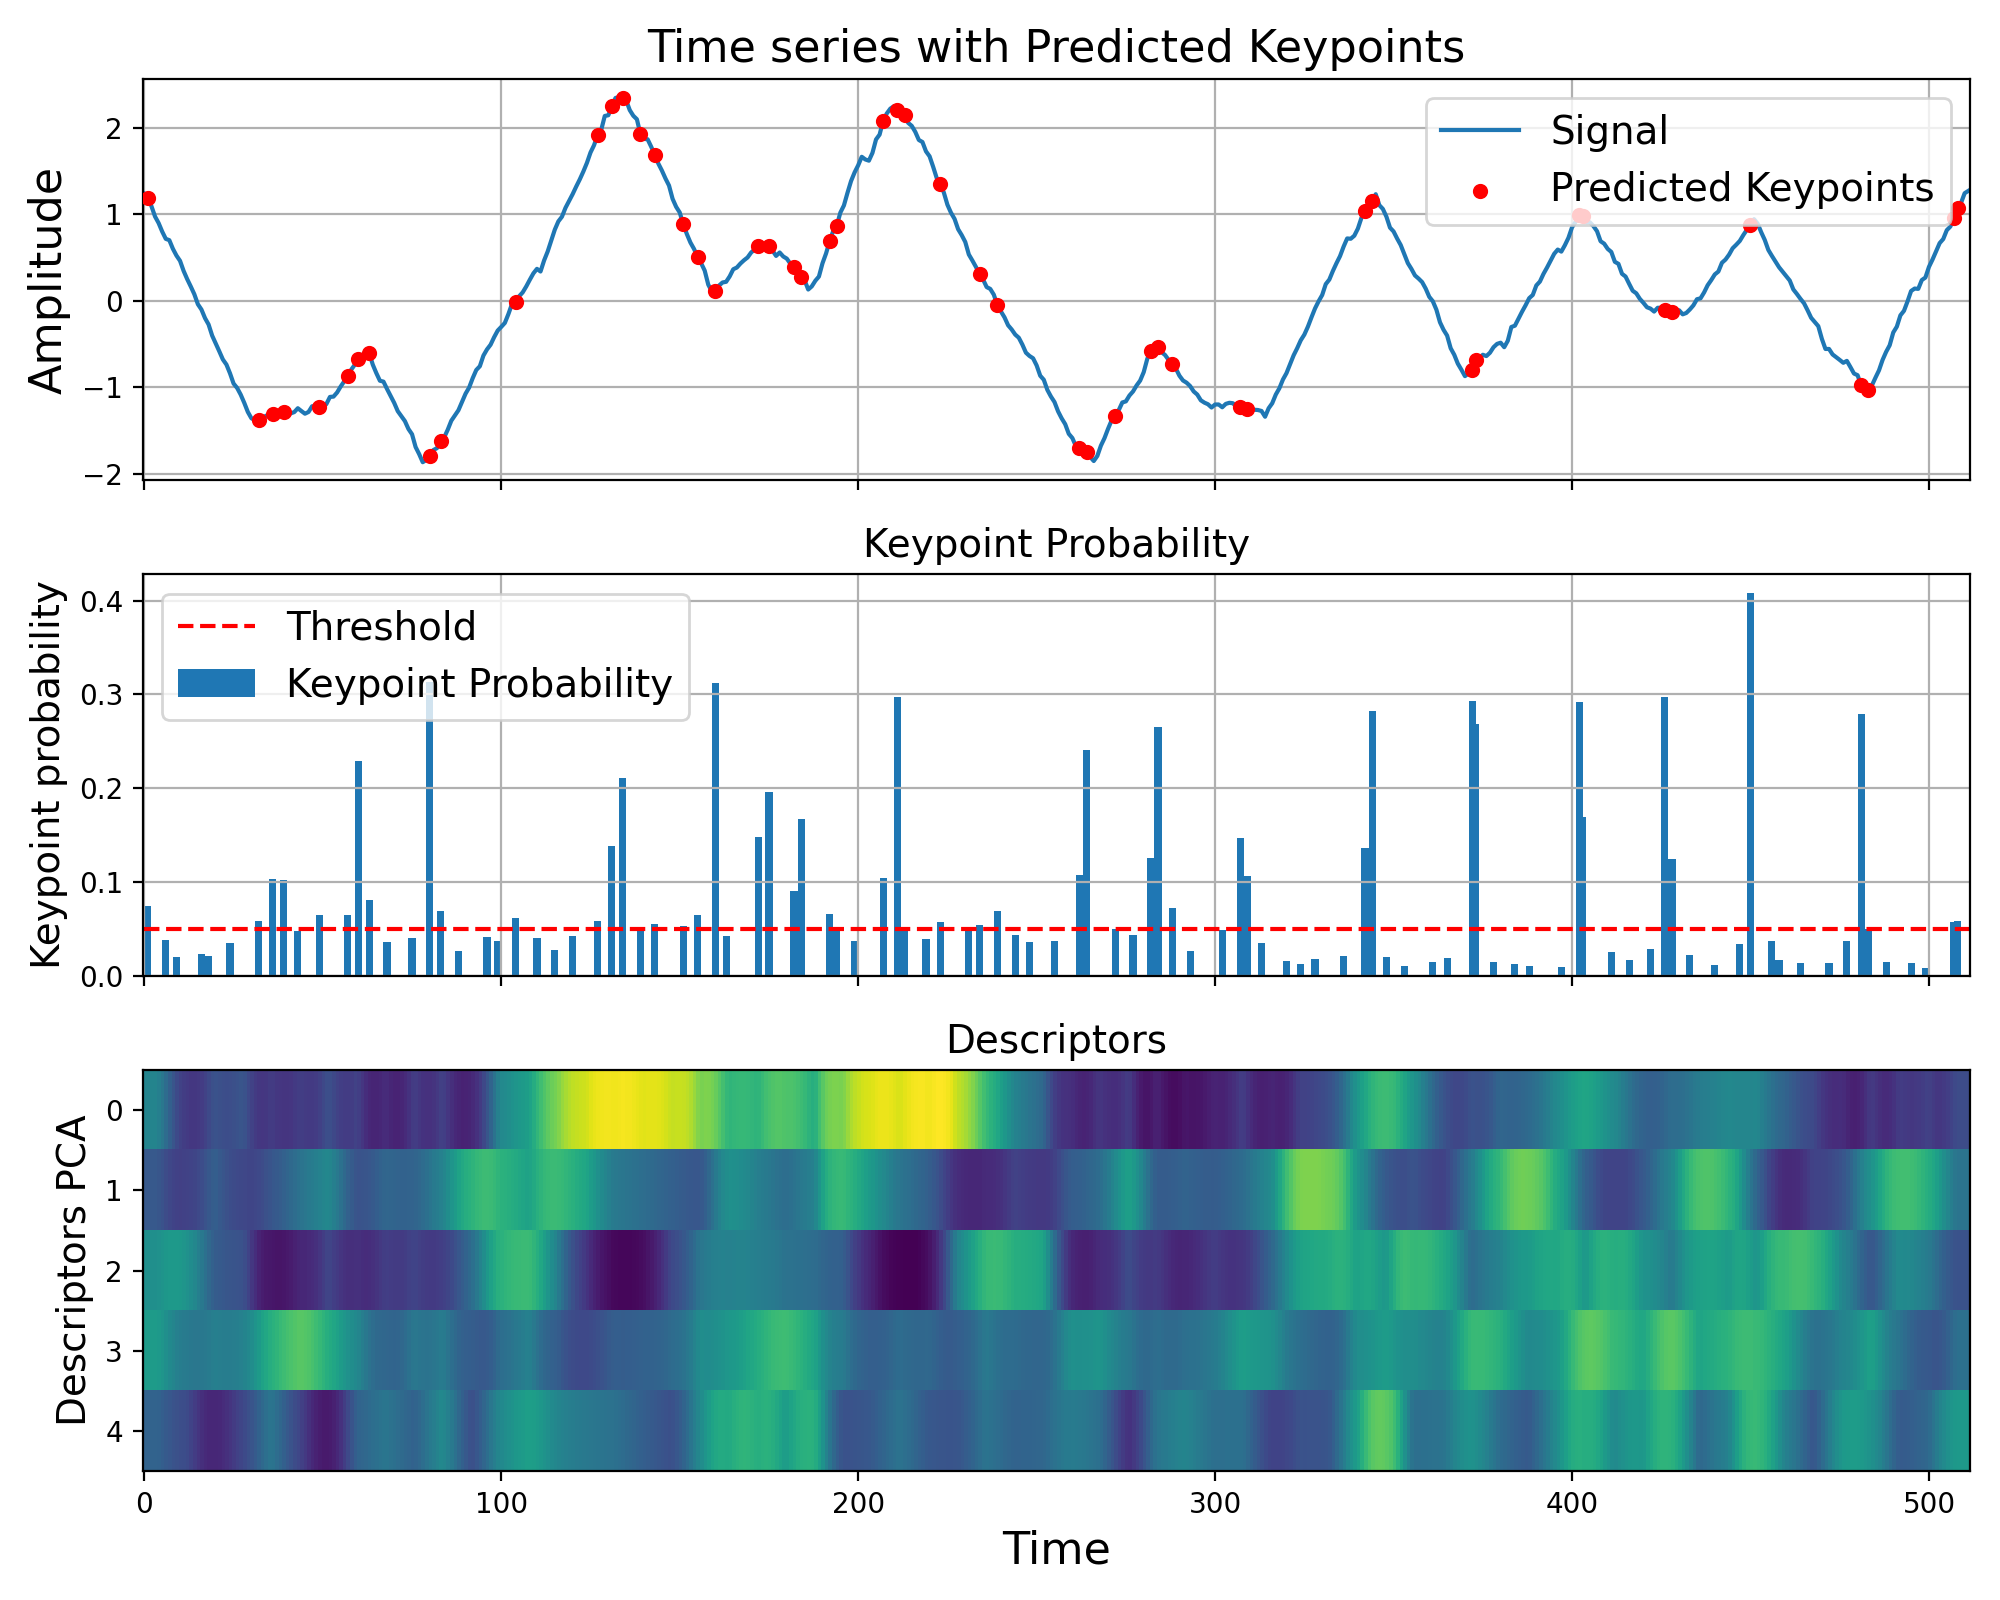}
    \includegraphics[width=0.49\linewidth]{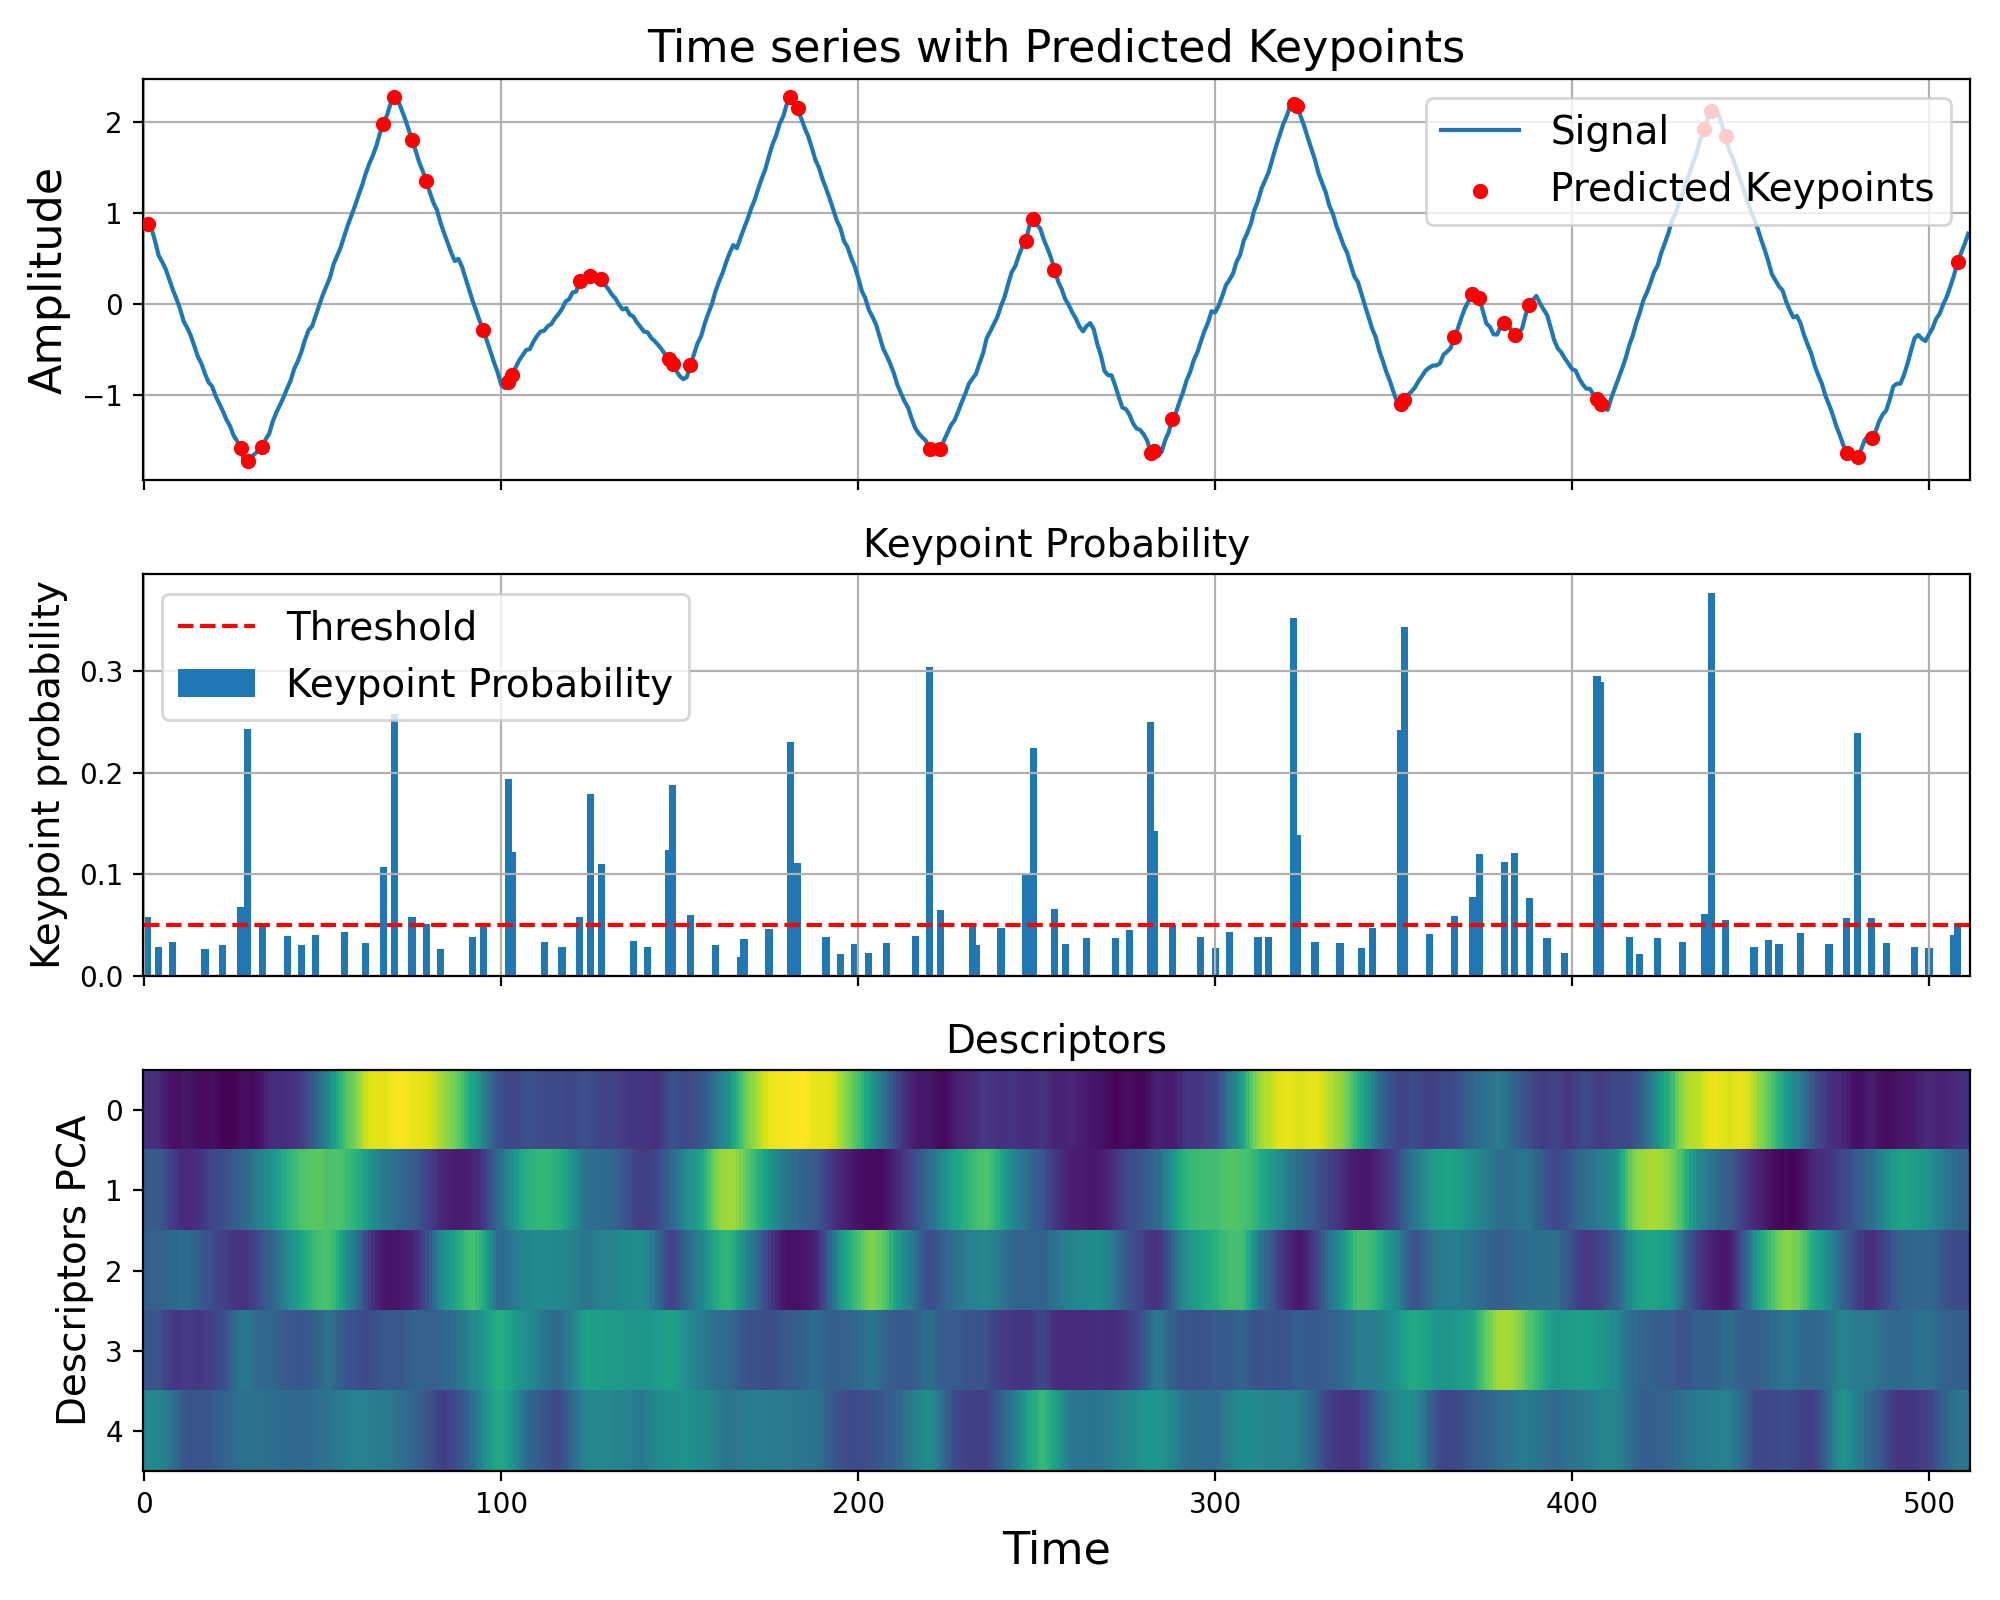}
    \caption{TimePoint Interest Point for the \texttt{BeetleFly} dataset}
    \label{fig:supmat:desc:kp:1}
\end{figure}
\begin{figure}
    \centering
    \includegraphics[width=0.49\linewidth]{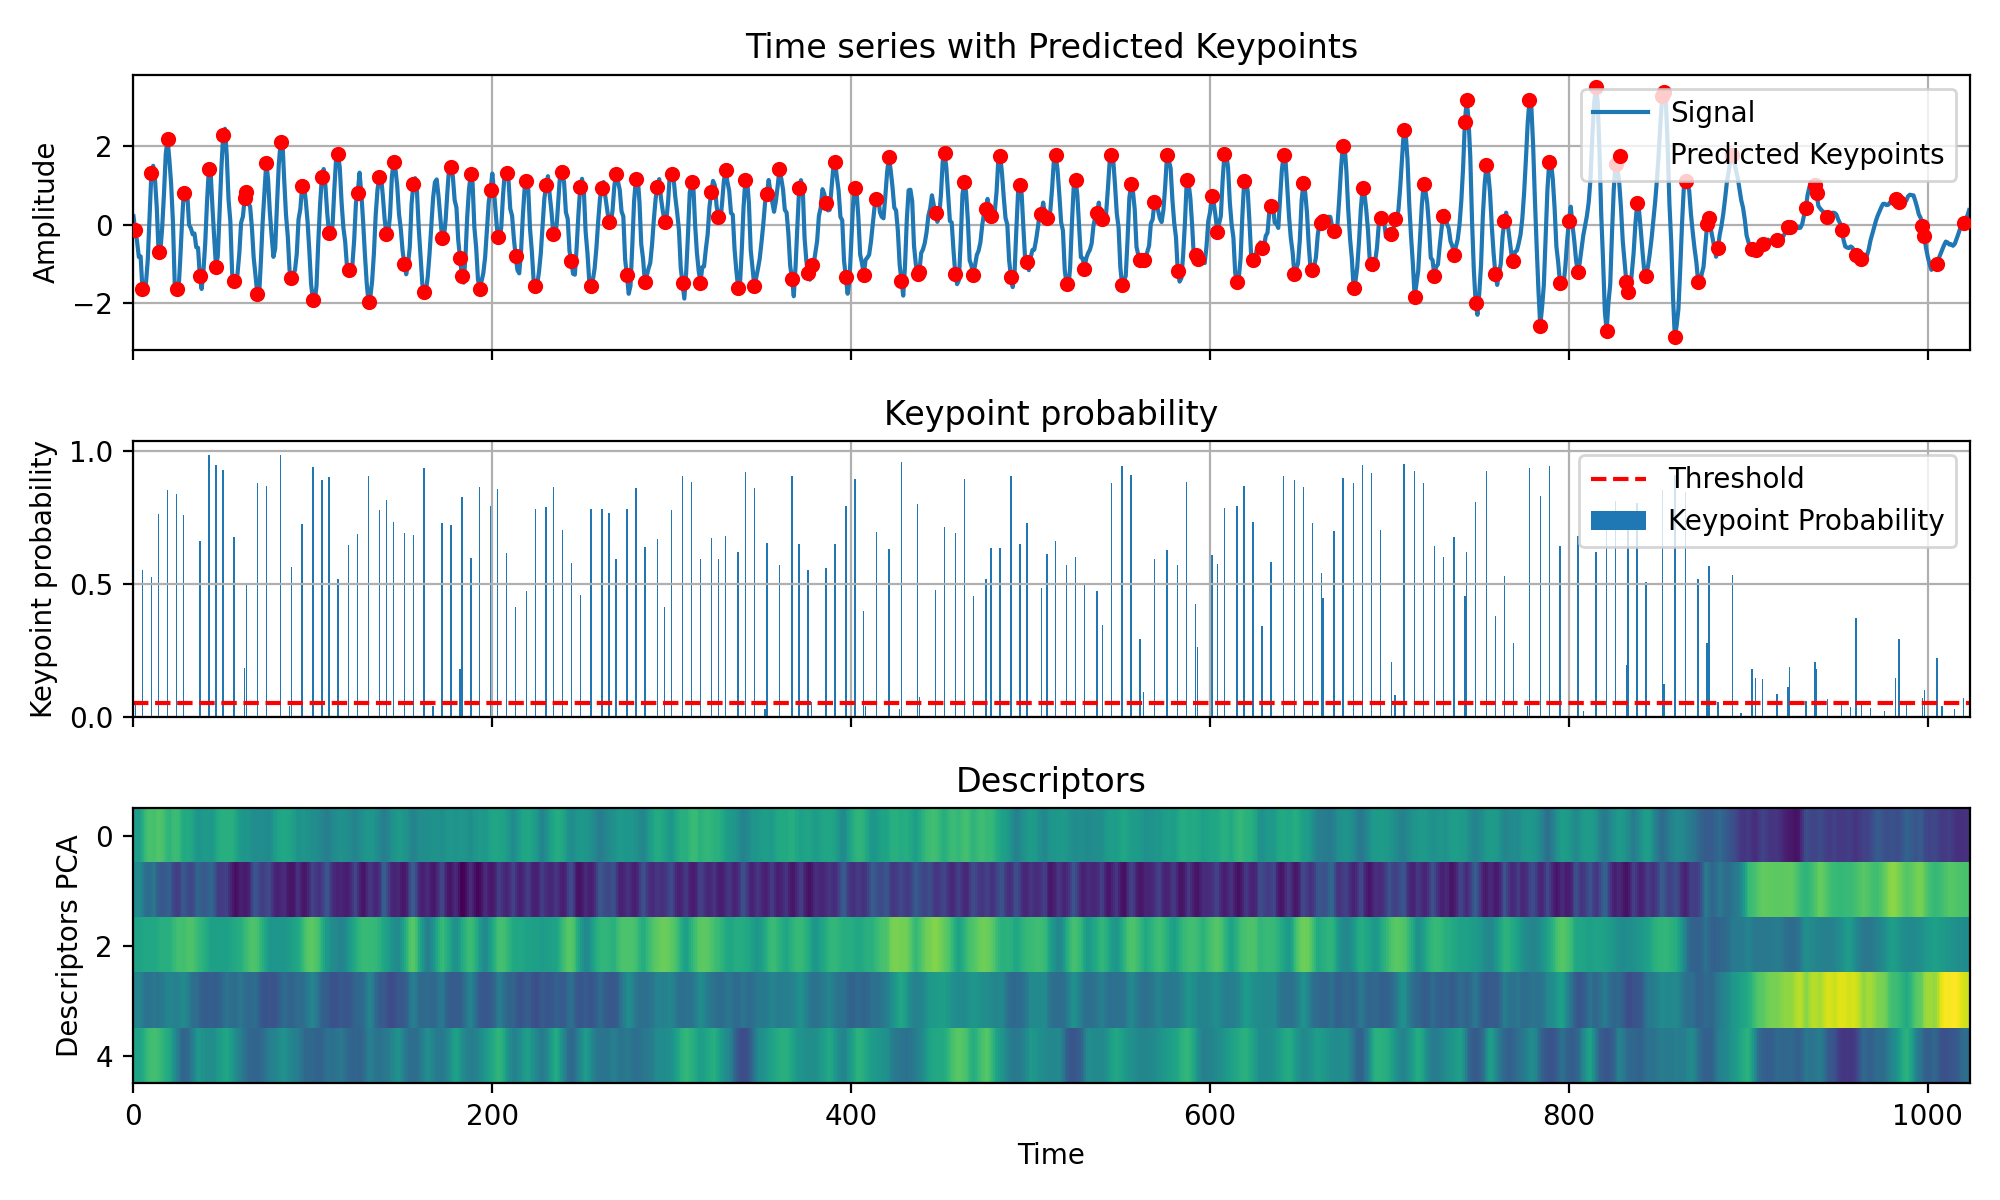}
    \includegraphics[width=0.49\linewidth]{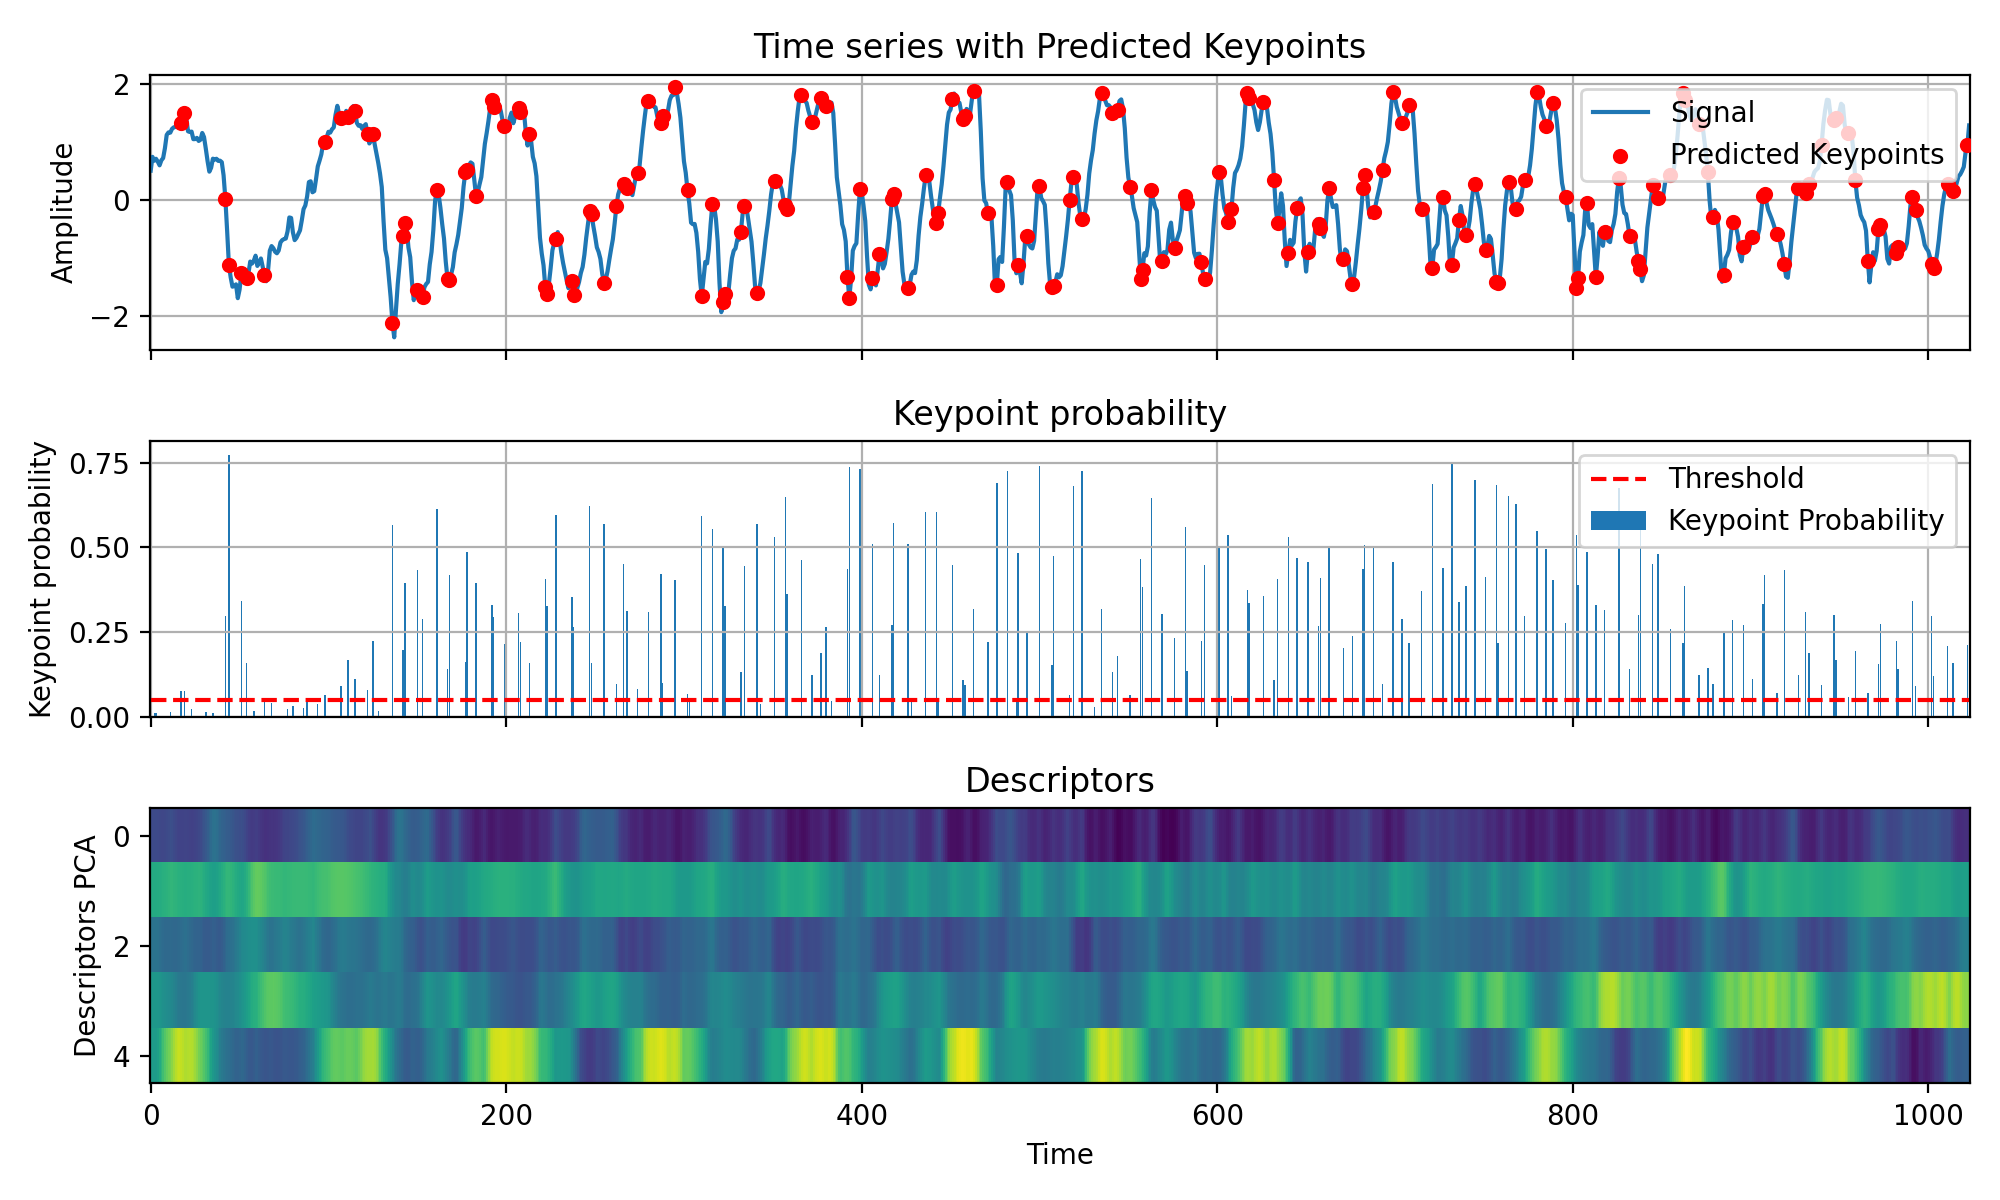}
    \caption{TimePoint Interest Point for the \texttt{Phoneme} dataset}
    \label{fig:supmat:desc:kp2}
\end{figure}
\begin{figure}
    \centering
    \includegraphics[width=0.49\linewidth]{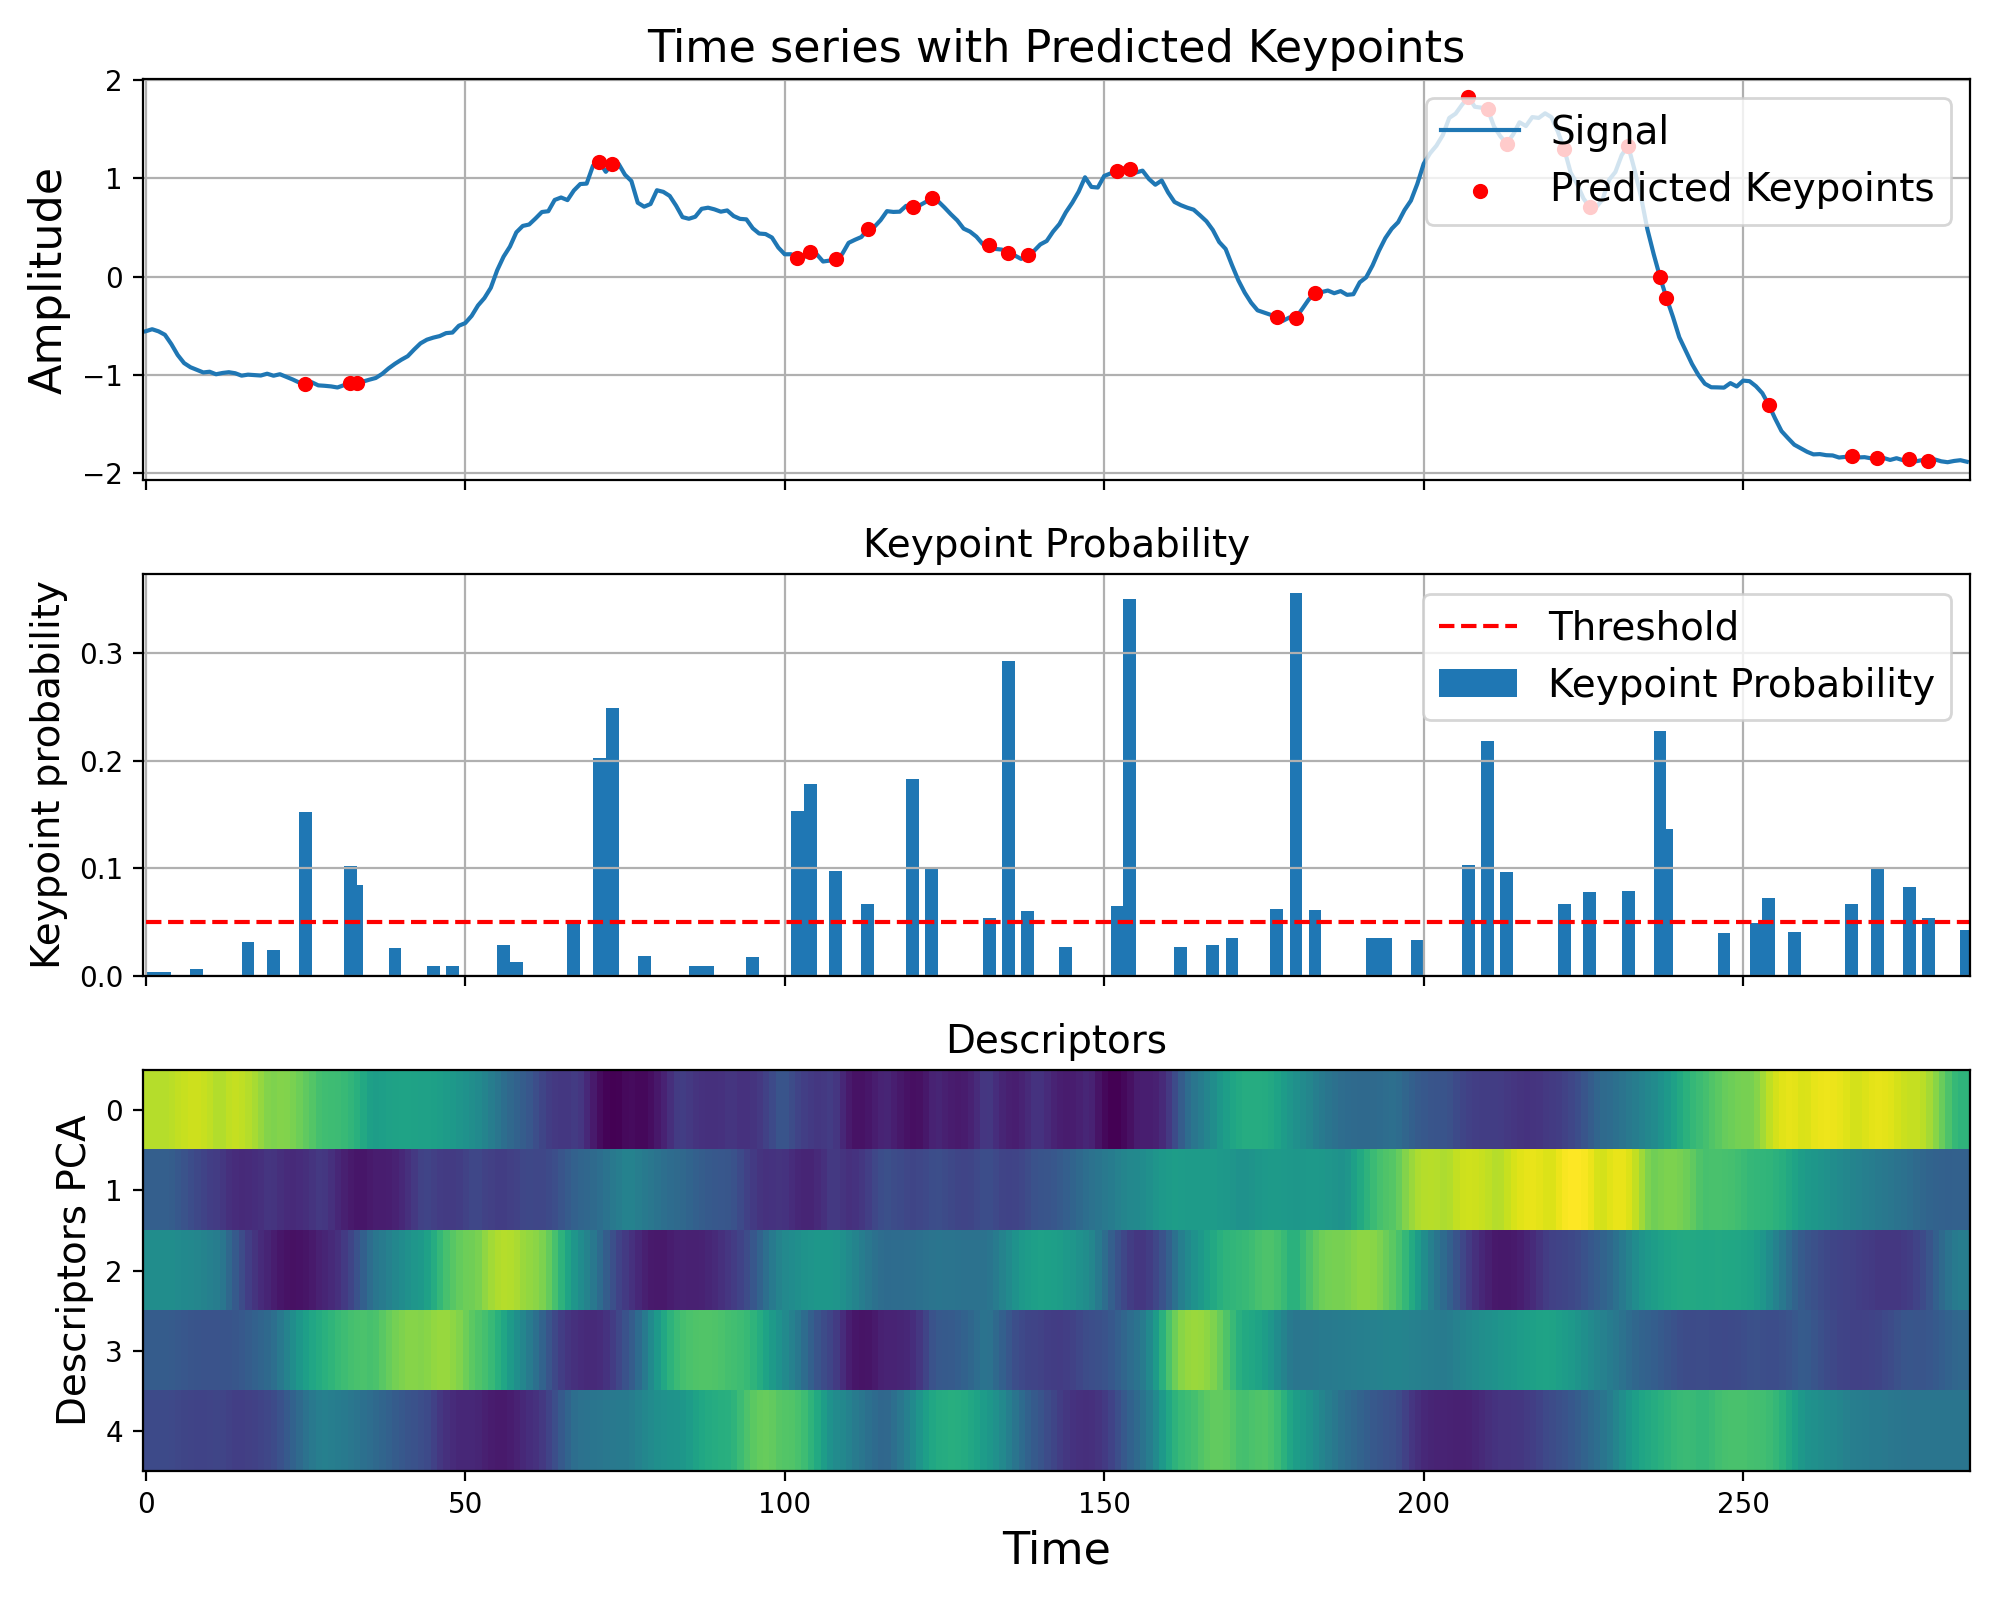}
    \includegraphics[width=0.49\linewidth]{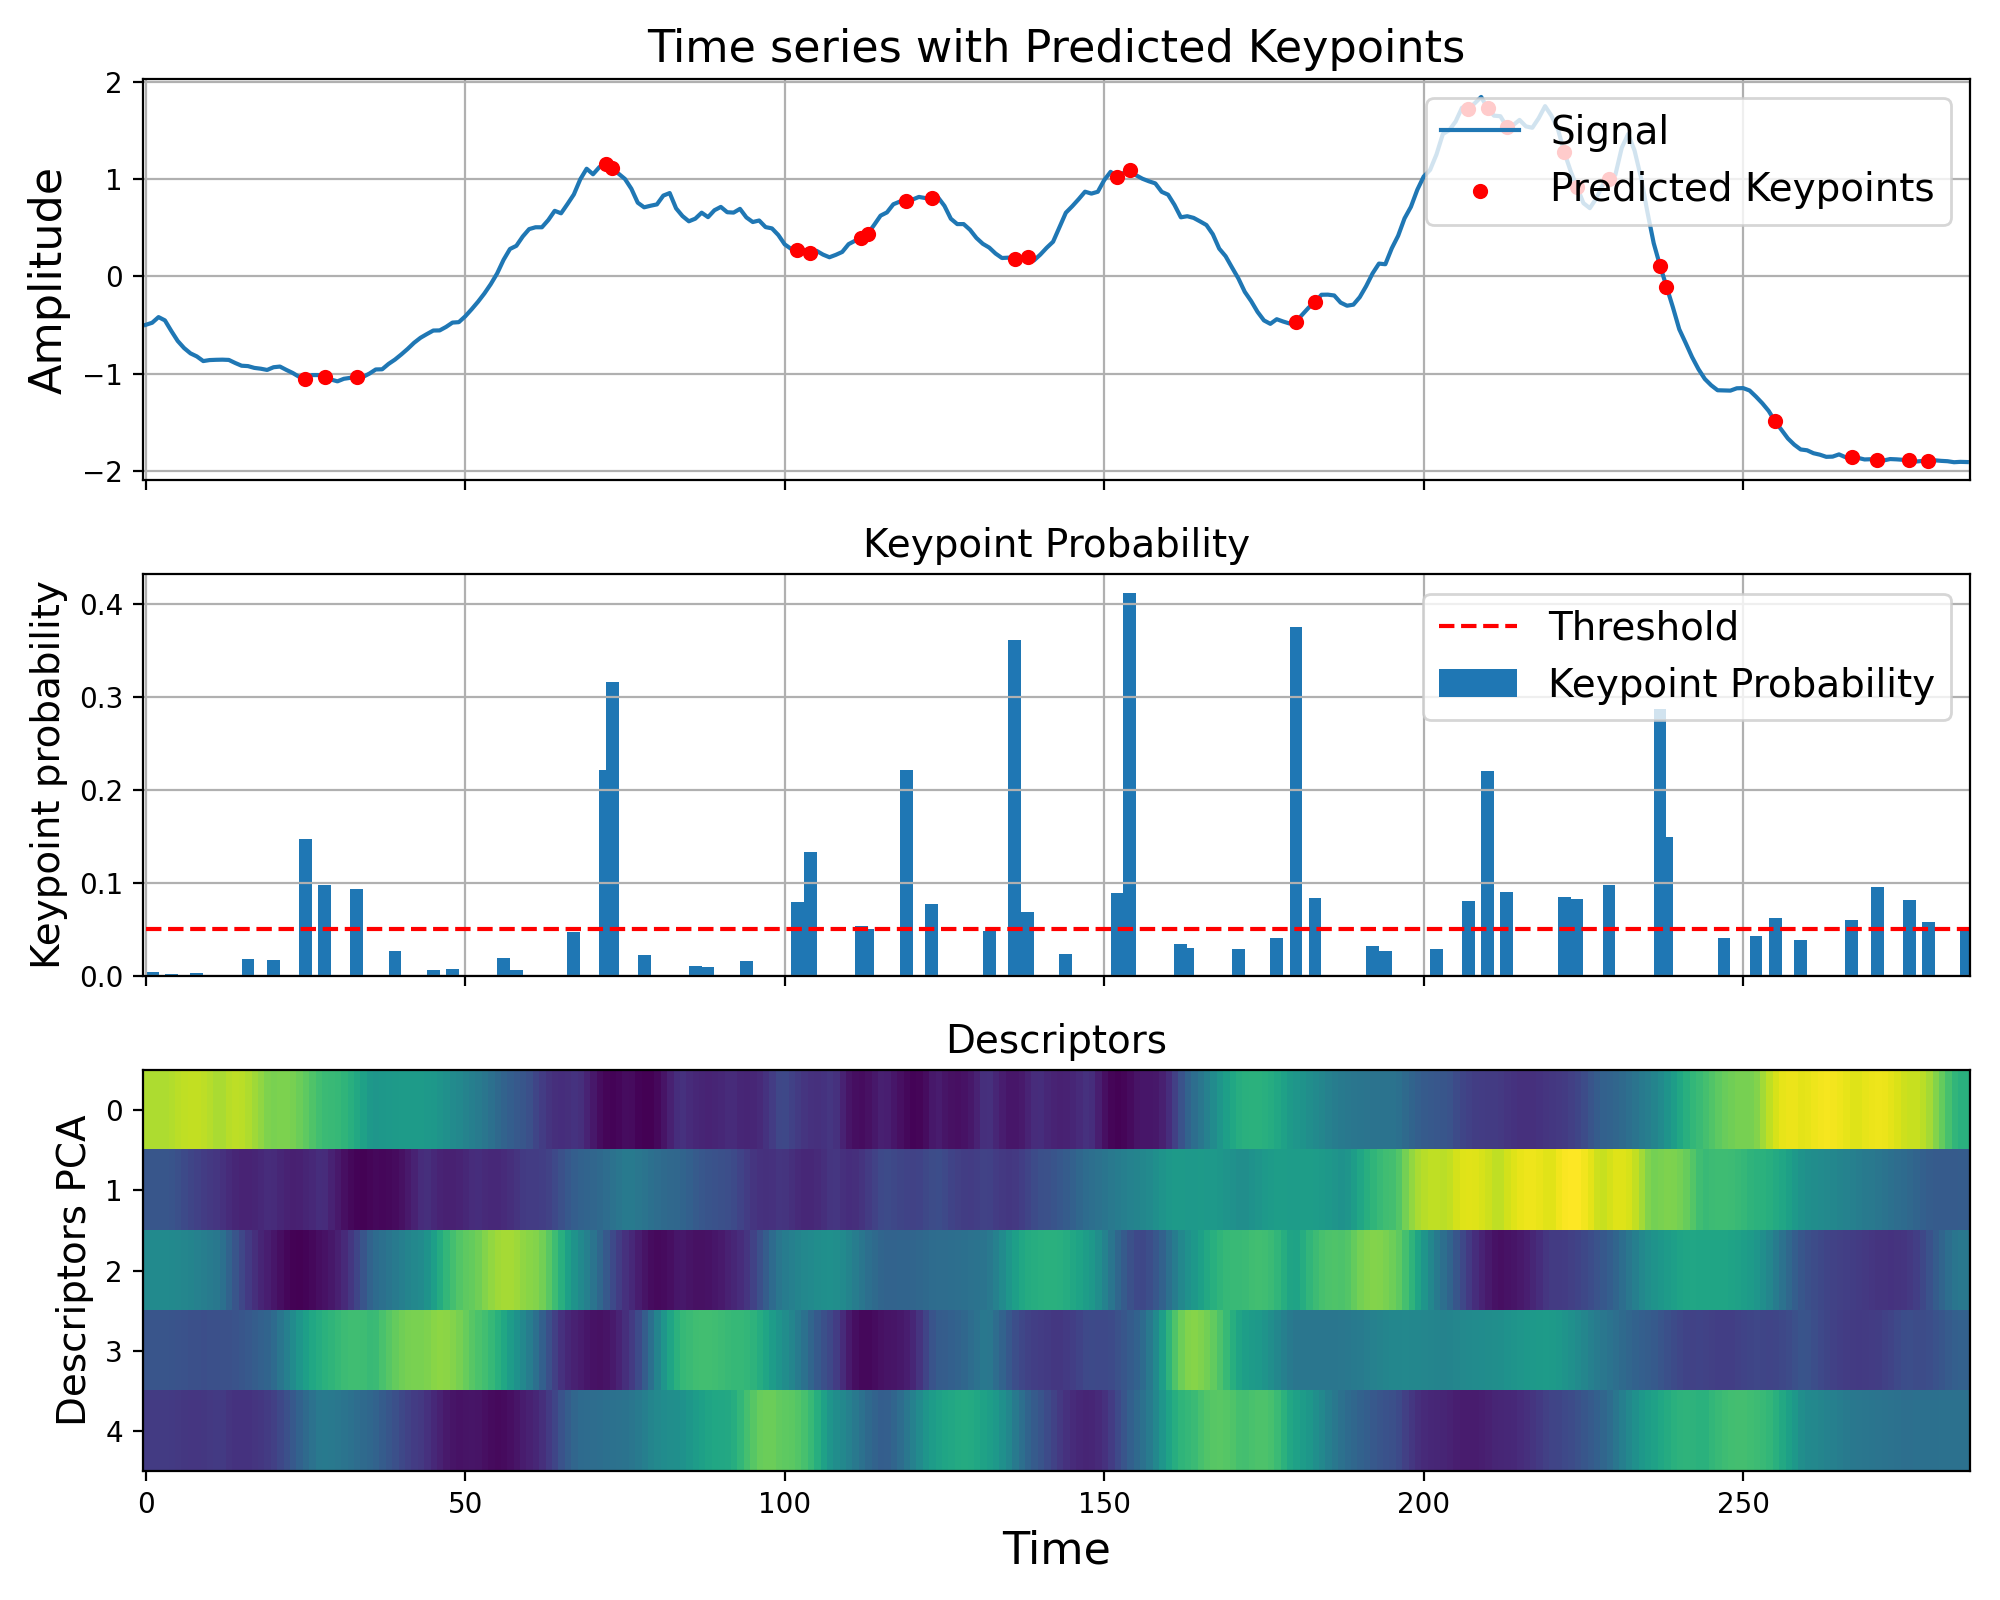}
    \caption{TimePoint Interest Point for the \texttt{Phoneme} dataset}
    \label{fig:supmat:desc:kp3}
\end{figure}
