# Supplementary material for: TimePoint: Accelerated Time Series Alignment via Self-Supervised Keypoint and Descriptor Learning
Source: arXiv:2505.23475 source file (2025-05-29)
Supplement: Supplementary file 3 [file all_ucr_tp100.pdf]

| TP         | Dataset                        | Keypoints Percentage | Accuracy | F1 Score | Precision | Recall |
|------------|--------------------------------|----------------------|----------|----------|-----------|--------|
| TP + Dense | SmoothSubspace                 | 1.0                  | 0.907    | 0.908    | 0.907     | 0.907  |
| TP + Dense | Chinatown                      | 1.0                  | 0.942    | 0.914    | 0.953     | 0.93   |
| TP + Dense | ItalyPowerDemand               | 1.0                  | 0.957    | 0.957    | 0.957     | 0.957  |
| TP + Dense | MelbournePedestrian            | 1.0                  | 0.1      | 0.01     | 0.1       | 0.018  |
| TP + Dense | Crop                           | 1.0                  | 0.699    | 0.682    | 0.699     | 0.688  |
| TP + Dense | SyntheticControl               | 1.0                  | 0.987    | 0.987    | 0.987     | 0.987  |
| TP + Dense | SonyAIBORobotSurface2          | 1.0                  | 0.873    | 0.864    | 0.875     | 0.868  |
| TP + Dense | SonyAIBORobotSurface1          | 1.0                  | 0.739    | 0.811    | 0.771     | 0.735  |
| TP + Dense | DistalPhalanxOutlineAgeGroup   | 1.0                  | 0.655    | 0.625    | 0.689     | 0.647  |
| TP + Dense | DistalPhalanxOutlineCorrect    | 1.0                  | 0.739    | 0.734    | 0.723     | 0.726  |
| TP + Dense | DistalPhalanxTW                | 1.0                  | 0.662    | 0.568    | 0.565     | 0.56   |
| TP + Dense | MiddlePhalanxOutlineAgeGroup   | 1.0                  | 0.435    | 0.413    | 0.43      | 0.408  |
| TP + Dense | MiddlePhalanxOutlineCorrect    | 1.0                  | 0.722    | 0.721    | 0.725     | 0.72   |
| TP + Dense | MiddlePhalanxTW                | 1.0                  | 0.552    | 0.427    | 0.428     | 0.426  |
| TP + Dense | PhalangesOutlinesCorrect       | 1.0                  | 0.761    | 0.75     | 0.738     | 0.743  |
| TP + Dense | ProximalPhalanxOutlineAgeGroup | 1.0                  | 0.805    | 0.714    | 0.757     | 0.727  |
| TP + Dense | ProximalPhalanxOutlineCorrect  | 1.0                  | 0.835    | 0.842    | 0.765     | 0.788  |
| TP + Dense | ProximalPhalanxTW              | 1.0                  | 0.741    | 0.505    | 0.537     | 0.499  |
| TP + Dense | TwoLeadECG                     | 1.0                  | 0.873    | 0.878    | 0.873     | 0.872  |
| TP + Dense | MoteStrain                     | 1.0                  | 0.889    | 0.891    | 0.886     | 0.888  |
| TP + Dense | ECG200                         | 1.0                  | 0.86     | 0.851    | 0.842     | 0.846  |
| TP + Dense | ElectricDevices                | 1.0                  | 0.611    | 0.544    | 0.496     | 0.507  |
| TP + Dense | MedicalImages                  | 1.0                  | 0.736    | 0.733    | 0.69      | 0.703  |

|            |             |     |       |       |       |       |
|------------|-------------|-----|-------|-------|-------|-------|
| TP + Dense | BME         | 1.0 | 0.927 | 0.94  | 0.927 | 0.927 |
| TP + Dense | CBF         | 1.0 | 1.0   | 1.0   | 1.0   | 1.0   |
| TP + Dense | SwedishLeaf | 1.0 | 0.926 | 0.931 | 0.929 | 0.928 |
| TP + Dense | TwoPatterns | 1.0 | 0.984 | 0.984 | 0.985 | 0.984 |
| TP + Dense | FaceAll     | 1.0 | 0.749 | 0.843 | 0.866 | 0.803 |
| TP + Dense | FacesUCR    | 1.0 | 0.913 | 0.91  | 0.887 | 0.894 |
| TP + Dense | ECGFiveDays | 1.0 | 0.729 | 0.772 | 0.731 | 0.719 |

| TP         | Dataset                  | Keypoints Percentage | Accuracy | F1 Score | Precision | Recall |
|------------|--------------------------|----------------------|----------|----------|-----------|--------|
| TP + Dense | ECG5000                  | 1.0                  | 0.929    | 0.674    | 0.569     | 0.596  |
| TP + Dense | Plane                    | 1.0                  | 1.0      | 1.0      | 1.0       | 1.0    |
| TP + Dense | PowerCons                | 1.0                  | 0.867    | 0.867    | 0.867     | 0.867  |
| TP + Dense | GunPoint                 | 1.0                  | 0.993    | 0.994    | 0.993     | 0.993  |
| TP + Dense | GunPointAgeSpan          | 1.0                  | 0.984    | 0.984    | 0.984     | 0.984  |
| TP + Dense | GunPointMaleVersusFemale | 1.0                  | 0.994    | 0.993    | 0.994     | 0.994  |
| TP + Dense | GunPointOldVersusYoung   | 1.0                  | 0.965    | 0.968    | 0.964     | 0.965  |
| TP + Dense | UMD                      | 1.0                  | 0.958    | 0.963    | 0.958     | 0.958  |
| TP + Dense | Wafer                    | 1.0                  | 0.983    | 0.978    | 0.932     | 0.954  |
| TP + Dense | ChlorineConcentration    | 1.0                  | 0.635    | 0.59     | 0.585     | 0.587  |
| TP + Dense | Adiac                    | 1.0                  | 0.716    | 0.74     | 0.71      | 0.702  |
| TP + Dense | Fungi                    | 1.0                  | 0.941    | 0.95     | 0.968     | 0.953  |
| TP + Dense | Wine                     | 1.0                  | 0.611    | 0.611    | 0.611     | 0.611  |
| TP + Dense | Strawberry               | 1.0                  | 0.954    | 0.945    | 0.958     | 0.951  |
| TP + Dense | ArrowHead                | 1.0                  | 0.817    | 0.832    | 0.832     | 0.819  |

|            |                      |     |       |       |       |       |
|------------|----------------------|-----|-------|-------|-------|-------|
| TP + Dense | InsectWingbeatSound  | 1.0 | 0.473 | 0.467 | 0.473 | 0.465 |
| TP + Dense | FiftyWords           | 1.0 | 0.78  | 0.675 | 0.664 | 0.656 |
| TP + Dense | WordSynonyms         | 1.0 | 0.74  | 0.698 | 0.627 | 0.633 |
| TP + Dense | Trace                | 1.0 | 1.0   | 1.0   | 1.0   | 1.0   |
| TP + Dense | ToeSegmentation1     | 1.0 | 0.873 | 0.888 | 0.868 | 0.87  |
| TP + Dense | Coffee               | 1.0 | 1.0   | 1.0   | 1.0   | 1.0   |
| TP + Dense | DodgerLoopDay        | 1.0 | 0.15  | 0.021 | 0.143 | 0.037 |
| TP + Dense | DodgerLoopGame       | 1.0 | 0.478 | 0.239 | 0.5   | 0.324 |
| TP + Dense | DodgerLoopWeekend    | 1.0 | 0.261 | 0.13  | 0.5   | 0.207 |
| TP + Dense | CricketX             | 1.0 | 0.744 | 0.752 | 0.746 | 0.746 |
| TP + Dense | CricketY             | 1.0 | 0.746 | 0.763 | 0.747 | 0.75  |
| TP + Dense | CricketZ             | 1.0 | 0.795 | 0.803 | 0.788 | 0.788 |
| TP + Dense | FreezerRegularTrain  | 1.0 | 0.921 | 0.921 | 0.921 | 0.921 |
| TP + Dense | FreezerSmallTrain    | 1.0 | 0.786 | 0.789 | 0.786 | 0.786 |
| TP + Dense | UWaveGestureLibraryX | 1.0 | 0.784 | 0.766 | 0.781 | 0.766 |

| TP         | Dataset              | Keypoints Percentage | Accuracy | F1 Score | Precision | Recall |
|------------|----------------------|----------------------|----------|----------|-----------|--------|
| TP + Dense | UWaveGestureLibraryY | 1.0                  | 0.703    | 0.706    | 0.704     | 0.7    |
| TP + Dense | UWaveGestureLibraryZ | 1.0                  | 0.706    | 0.693    | 0.708     | 0.69   |
| TP + Dense | Lightning7           | 1.0                  | 0.726    | 0.761    | 0.73      | 0.732  |
| TP + Dense | ToeSegmentation2     | 1.0                  | 0.946    | 0.892    | 0.951     | 0.917  |
| TP + Dense | DiatomSizeReduction  | 1.0                  | 0.964    | 0.974    | 0.917     | 0.936  |
| TP + Dense | FaceFour             | 1.0                  | 0.92     | 0.918    | 0.929     | 0.918  |
| TP + Dense | GestureMidAirD1      | 1.0                  | 0.038    | 0.001    | 0.038     | 0.003  |

|            |                       |     |       |       |       |       |
|------------|-----------------------|-----|-------|-------|-------|-------|
| TP + Dense | GestureMidAirD2       | 1.0 | 0.038 | 0.001 | 0.038 | 0.003 |
| TP + Dense | GestureMidAirD3       | 1.0 | 0.038 | 0.001 | 0.038 | 0.003 |
| TP + Dense | PickupGestureWiimoteZ | 1.0 | 0.1   | 0.01  | 0.1   | 0.018 |
| TP + Dense | AllGestureWiimoteX    | 1.0 | 0.1   | 0.01  | 0.1   | 0.018 |
| TP + Dense | AllGestureWiimoteY    | 1.0 | 0.1   | 0.01  | 0.1   | 0.018 |
| TP + Dense | AllGestureWiimoteZ    | 1.0 | 0.1   | 0.01  | 0.1   | 0.018 |
| TP + Dense | ShakeGestureWiimoteZ  | 1.0 | 0.1   | 0.01  | 0.1   | 0.018 |
| TP + Dense | Symbols               | 1.0 | 0.966 | 0.97  | 0.964 | 0.966 |
| TP + Dense | Yoga                  | 1.0 | 0.881 | 0.882 | 0.878 | 0.879 |
| TP + Dense | OSULeaf               | 1.0 | 0.802 | 0.822 | 0.808 | 0.805 |
| TP + Dense | Ham                   | 1.0 | 0.552 | 0.554 | 0.553 | 0.552 |
| TP + Dense | Meat                  | 1.0 | 0.9   | 0.909 | 0.9   | 0.899 |
| TP + Dense | GesturePebbleZ1       | 1.0 | 0.163 | 0.027 | 0.167 | 0.047 |
| TP + Dense | GesturePebbleZ2       | 1.0 | 0.152 | 0.025 | 0.167 | 0.044 |
| TP + Dense | Fish                  | 1.0 | 0.931 | 0.932 | 0.932 | 0.929 |
| TP + Dense | Beef                  | 1.0 | 0.7   | 0.774 | 0.7   | 0.693 |
| TP + Dense | FordA                 | 1.0 | 0.786 | 0.788 | 0.784 | 0.784 |
| TP + Dense | FordB                 | 1.0 | 0.701 | 0.701 | 0.701 | 0.701 |
| TP + Dense | ShapeletSim           | 1.0 | 0.706 | 0.717 | 0.706 | 0.701 |
| TP + Dense | BeetleFly             | 1.0 | 0.65  | 0.794 | 0.65  | 0.601 |
| TP + Dense | BirdChicken           | 1.0 | 0.8   | 0.8   | 0.8   | 0.8   |
| TP + Dense | Earthquakes           | 1.0 | 0.763 | 0.675 | 0.633 | 0.645 |
| TP + Dense | Herring               | 1.0 | 0.484 | 0.469 | 0.469 | 0.469 |

| TP          | Dataset                    | Keypoints Percentage | Accuracy | F1 Score | Precision | Recall |
|-------------|----------------------------|----------------------|----------|----------|-----------|--------|
| TP + Dense  | ShapesAll                  | 1.0                  | 0.86     | 0.881    | 0.86      | 0.856  |
| TP + Dense  | OliveOil                   | 1.0                  | 0.867    | 0.85     | 0.804     | 0.819  |
| TP + Dense  | Car                        | 1.0                  | 0.833    | 0.88     | 0.814     | 0.794  |
| TP + Dense  | InsectEPGRegularTrain      | 1.0                  | 0.912    | 0.897    | 0.897     | 0.897  |
| TP + Dense  | InsectEPGSmallTrain        | 1.0                  | 0.815    | 0.791    | 0.82      | 0.795  |
| TP + Dense  | Lightning2                 | 1.0                  | 0.885    | 0.891    | 0.88      | 0.883  |
| TP + Dense  | Computers                  | 1.0                  | 0.62     | 0.62     | 0.62      | 0.62   |
| TP + Dense  | LargeKitchenAppliances     | 1.0                  | 0.795    | 0.802    | 0.795     | 0.795  |
| TP + Dense  | RefrigerationDevices       | 1.0                  | 0.477    | 0.489    | 0.477     | 0.481  |
| TP + Dense  | ScreenType                 | 1.0                  | 0.397    | 0.402    | 0.397     | 0.396  |
| TP + Dense  | SmallKitchenAppliances     | 1.0                  | 0.64     | 0.646    | 0.64      | 0.638  |
| TP + Dense  | NonInvasiveFetalECGThorax1 | 1.0                  | 0.744    | 0.766    | 0.741     | 0.732  |
| TP + Dense  | NonInvasiveFetalECGThorax2 | 1.0                  | 0.83     | 0.83     | 0.825     | 0.82   |
| TP + Dense  | Worms                      | 1.0                  | 0.623    | 0.689    | 0.6       | 0.622  |
| TP + Dense  | WormsTwoClass              | 1.0                  | 0.727    | 0.722    | 0.723     | 0.723  |
| TP + WTConv | SmoothSubspace             | 1.0                  | 0.813    | 0.819    | 0.813     | 0.809  |
| TP + WTConv | Chinatown                  | 1.0                  | 0.945    | 0.918    | 0.955     | 0.934  |
| TP + WTConv | ItalyPowerDemand           | 1.0                  | 0.945    | 0.945    | 0.945     | 0.945  |
| TP + WTConv | MelbournePedestrian        | 1.0                  | 0.1      | 0.01     | 0.1       | 0.018  |
| TP + WTConv | Crop                       | 1.0                  | 0.705    | 0.69     | 0.705     | 0.694  |
| TP + WTConv | SyntheticControl           | 1.0                  | 0.983    | 0.984    | 0.983     | 0.983  |
| TP + WTConv | SonyAIBORobotSurface2      | 1.0                  | 0.866    | 0.866    | 0.847     | 0.854  |
| TP + WTConv | SonyAIBORobotSurface1      | 1.0                  | 0.745    | 0.814    | 0.777     | 0.742  |

|             |                              |     |       |       |       |       |
|-------------|------------------------------|-----|-------|-------|-------|-------|
| TP + WTConv | DistalPhalanxOutlineAgeGroup | 1.0 | 0.583 | 0.527 | 0.567 | 0.535 |
| TP + WTConv | DistalPhalanxOutlineCorrect  | 1.0 | 0.717 | 0.71  | 0.701 | 0.703 |
| TP + WTConv | DistalPhalanxTW              | 1.0 | 0.59  | 0.462 | 0.47  | 0.463 |
| TP + WTConv | MiddlePhalanxOutlineAgeGroup | 1.0 | 0.396 | 0.36  | 0.361 | 0.354 |
| TP + WTConv | MiddlePhalanxOutlineCorrect  | 1.0 | 0.722 | 0.719 | 0.722 | 0.719 |
| TP + WTConv | MiddlePhalanxTW              | 1.0 | 0.539 | 0.424 | 0.414 | 0.416 |
| TP + WTConv | PhalangesOutlinesCorrect     | 1.0 | 0.741 | 0.727 | 0.724 | 0.725 |

| TP          | Dataset                        | Keypoints Percentage | Accuracy | F1 Score | Precision | Recall |
|-------------|--------------------------------|----------------------|----------|----------|-----------|--------|
| TP + WTConv | ProximalPhalanxOutlineAgeGroup | 1.0                  | 0.795    | 0.715    | 0.735     | 0.723  |
| TP + WTConv | ProximalPhalanxOutlineCorrect  | 1.0                  | 0.852    | 0.87     | 0.784     | 0.809  |
| TP + WTConv | ProximalPhalanxTW              | 1.0                  | 0.727    | 0.47     | 0.518     | 0.47   |
| TP + WTConv | TwoLeadECG                     | 1.0                  | 0.834    | 0.842    | 0.834     | 0.833  |
| TP + WTConv | MoteStrain                     | 1.0                  | 0.862    | 0.865    | 0.858     | 0.86   |
| TP + WTConv | ECG200                         | 1.0                  | 0.82     | 0.828    | 0.774     | 0.79   |
| TP + WTConv | ElectricDevices                | 1.0                  | 0.613    | 0.563    | 0.529     | 0.538  |
| TP + WTConv | MedicalImages                  | 1.0                  | 0.728    | 0.725    | 0.708     | 0.709  |
| TP + WTConv | BME                            | 1.0                  | 0.953    | 0.959    | 0.953     | 0.954  |
| TP + WTConv | CBF                            | 1.0                  | 0.993    | 0.993    | 0.993     | 0.993  |
| TP + WTConv | SwedishLeaf                    | 1.0                  | 0.899    | 0.908    | 0.902     | 0.9    |
| TP + WTConv | TwoPatterns                    | 1.0                  | 0.778    | 0.779    | 0.778     | 0.778  |
| TP + WTConv | FaceAll                        | 1.0                  | 0.734    | 0.791    | 0.835     | 0.764  |
| TP + WTConv | FacesUCR                       | 1.0                  | 0.859    | 0.862    | 0.82      | 0.832  |
| TP + WTConv | ECGFiveDays                    | 1.0                  | 0.897    | 0.903    | 0.897     | 0.896  |

|             |                          |     |       |       |       |       |
|-------------|--------------------------|-----|-------|-------|-------|-------|
| TP + WTConv | ECG5000                  | 1.0 | 0.924 | 0.68  | 0.559 | 0.577 |
| TP + WTConv | Plane                    | 1.0 | 1.0   | 1.0   | 1.0   | 1.0   |
| TP + WTConv | PowerCons                | 1.0 | 0.894 | 0.9   | 0.894 | 0.894 |
| TP + WTConv | GunPoint                 | 1.0 | 0.993 | 0.994 | 0.993 | 0.993 |
| TP + WTConv | GunPointAgeSpan          | 1.0 | 0.978 | 0.978 | 0.978 | 0.978 |
| TP + WTConv | GunPointMaleVersusFemale | 1.0 | 1.0   | 1.0   | 1.0   | 1.0   |
| TP + WTConv | GunPointOldVersusYoung   | 1.0 | 0.981 | 0.982 | 0.98  | 0.981 |
| TP + WTConv | UMD                      | 1.0 | 0.889 | 0.888 | 0.889 | 0.887 |
| TP + WTConv | Wafer                    | 1.0 | 0.994 | 0.985 | 0.985 | 0.985 |
| TP + WTConv | ChlorineConcentration    | 1.0 | 0.632 | 0.59  | 0.584 | 0.586 |
| TP + WTConv | Adiac                    | 1.0 | 0.742 | 0.758 | 0.739 | 0.727 |
| TP + WTConv | Fungi                    | 1.0 | 0.995 | 0.995 | 0.997 | 0.996 |
| TP + WTConv | Wine                     | 1.0 | 0.593 | 0.593 | 0.593 | 0.592 |
| TP + WTConv | Strawberry               | 1.0 | 0.949 | 0.939 | 0.953 | 0.945 |
| TP + WTConv | ArrowHead                | 1.0 | 0.857 | 0.858 | 0.865 | 0.857 |

| TP          | Dataset             | Keypoints Percentage | Accuracy | F1 Score | Precision | Recall |
|-------------|---------------------|----------------------|----------|----------|-----------|--------|
| TP + WTConv | InsectWingbeatSound | 1.0                  | 0.534    | 0.533    | 0.534     | 0.532  |
| TP + WTConv | FiftyWords          | 1.0                  | 0.802    | 0.732    | 0.7       | 0.689  |
| TP + WTConv | WordSynonyms        | 1.0                  | 0.737    | 0.671    | 0.615     | 0.624  |
| TP + WTConv | Trace               | 1.0                  | 0.99     | 0.988    | 0.991     | 0.989  |
| TP + WTConv | ToeSegmentation1    | 1.0                  | 0.882    | 0.884    | 0.88      | 0.881  |
| TP + WTConv | Coffee              | 1.0                  | 1.0      | 1.0      | 1.0       | 1.0    |
| TP + WTConv | DodgerLoopDay       | 1.0                  | 0.15     | 0.021    | 0.143     | 0.037  |

|             |                       |     |       |       |       |       |
|-------------|-----------------------|-----|-------|-------|-------|-------|
| TP + WTConv | DodgerLoopGame        | 1.0 | 0.478 | 0.239 | 0.5   | 0.324 |
| TP + WTConv | DodgerLoopWeekend     | 1.0 | 0.261 | 0.13  | 0.5   | 0.207 |
| TP + WTConv | CricketX              | 1.0 | 0.754 | 0.774 | 0.761 | 0.761 |
| TP + WTConv | CricketY              | 1.0 | 0.759 | 0.778 | 0.757 | 0.761 |
| TP + WTConv | CricketZ              | 1.0 | 0.756 | 0.765 | 0.749 | 0.75  |
| TP + WTConv | FreezerRegularTrain   | 1.0 | 0.924 | 0.924 | 0.924 | 0.924 |
| TP + WTConv | FreezerSmallTrain     | 1.0 | 0.798 | 0.8   | 0.798 | 0.798 |
| TP + WTConv | UWaveGestureLibraryX  | 1.0 | 0.797 | 0.784 | 0.794 | 0.787 |
| TP + WTConv | UWaveGestureLibraryY  | 1.0 | 0.743 | 0.74  | 0.744 | 0.738 |
| TP + WTConv | UWaveGestureLibraryZ  | 1.0 | 0.738 | 0.726 | 0.739 | 0.727 |
| TP + WTConv | Lightning7            | 1.0 | 0.767 | 0.8   | 0.782 | 0.777 |
| TP + WTConv | ToeSegmentation2      | 1.0 | 0.9   | 0.823 | 0.906 | 0.854 |
| TP + WTConv | DiatomSizeReduction   | 1.0 | 0.958 | 0.968 | 0.902 | 0.922 |
| TP + WTConv | FaceFour              | 1.0 | 0.932 | 0.929 | 0.939 | 0.93  |
| TP + WTConv | GestureMidAirD1       | 1.0 | 0.038 | 0.001 | 0.038 | 0.003 |
| TP + WTConv | GestureMidAirD2       | 1.0 | 0.038 | 0.001 | 0.038 | 0.003 |
| TP + WTConv | GestureMidAirD3       | 1.0 | 0.038 | 0.001 | 0.038 | 0.003 |
| TP + WTConv | PickupGestureWiimoteZ | 1.0 | 0.1   | 0.01  | 0.1   | 0.018 |
| TP + WTConv | AllGestureWiimoteX    | 1.0 | 0.1   | 0.01  | 0.1   | 0.018 |
| TP + WTConv | AllGestureWiimoteY    | 1.0 | 0.1   | 0.01  | 0.1   | 0.018 |
| TP + WTConv | AllGestureWiimoteZ    | 1.0 | 0.1   | 0.01  | 0.1   | 0.018 |
| TP + WTConv | ShakeGestureWiimoteZ  | 1.0 | 0.1   | 0.01  | 0.1   | 0.018 |
| TP + WTConv | Symbols               | 1.0 | 0.965 | 0.967 | 0.964 | 0.965 |

| TP          | Dataset                | Keypoints Percentage | Accuracy | F1 Score | Precision | Recall |
|-------------|------------------------|----------------------|----------|----------|-----------|--------|
| TP + WTConv | Yoga                   | 1.0                  | 0.871    | 0.872    | 0.868     | 0.869  |
| TP + WTConv | OSULeaf                | 1.0                  | 0.81     | 0.836    | 0.816     | 0.816  |
| TP + WTConv | Ham                    | 1.0                  | 0.552    | 0.552    | 0.552     | 0.552  |
| TP + WTConv | Meat                   | 1.0                  | 0.917    | 0.922    | 0.917     | 0.916  |
| TP + WTConv | GesturePebbleZ1        | 1.0                  | 0.163    | 0.027    | 0.167     | 0.047  |
| TP + WTConv | GesturePebbleZ2        | 1.0                  | 0.152    | 0.025    | 0.167     | 0.044  |
| TP + WTConv | Fish                   | 1.0                  | 0.914    | 0.915    | 0.918     | 0.915  |
| TP + WTConv | Beef                   | 1.0                  | 0.8      | 0.819    | 0.8       | 0.805  |
| TP + WTConv | FordA                  | 1.0                  | 0.791    | 0.8      | 0.788     | 0.788  |
| TP + WTConv | FordB                  | 1.0                  | 0.662    | 0.664    | 0.662     | 0.661  |
| TP + WTConv | ShapeletSim            | 1.0                  | 0.711    | 0.738    | 0.711     | 0.703  |
| TP + WTConv | BeetleFly              | 1.0                  | 0.9      | 0.917    | 0.9       | 0.899  |
| TP + WTConv | BirdChicken            | 1.0                  | 0.85     | 0.885    | 0.85      | 0.847  |
| TP + WTConv | Earthquakes            | 1.0                  | 0.691    | 0.549    | 0.537     | 0.537  |
| TP + WTConv | Herring                | 1.0                  | 0.531    | 0.525    | 0.526     | 0.524  |
| TP + WTConv | ShapesAll              | 1.0                  | 0.878    | 0.896    | 0.878     | 0.874  |
| TP + WTConv | OliveOil               | 1.0                  | 0.933    | 0.955    | 0.917     | 0.928  |
| TP + WTConv | Car                    | 1.0                  | 0.867    | 0.867    | 0.867     | 0.867  |
| TP + WTConv | InsectEPGRegularTrain  | 1.0                  | 0.928    | 0.92     | 0.904     | 0.911  |
| TP + WTConv | InsectEPGSmallTrain    | 1.0                  | 0.803    | 0.78     | 0.811     | 0.785  |
| TP + WTConv | Lightning2             | 1.0                  | 0.82     | 0.818    | 0.82      | 0.819  |
| TP + WTConv | Computers              | 1.0                  | 0.676    | 0.676    | 0.676     | 0.676  |
| TP + WTConv | LargeKitchenAppliances | 1.0                  | 0.755    | 0.755    | 0.755     | 0.754  |

|             |                            |     |       |       |       |       |
|-------------|----------------------------|-----|-------|-------|-------|-------|
| TP + WTConv | RefrigerationDevices       | 1.0 | 0.483 | 0.496 | 0.483 | 0.486 |
| TP + WTConv | ScreenType                 | 1.0 | 0.416 | 0.416 | 0.416 | 0.415 |
| TP + WTConv | SmallKitchenAppliances     | 1.0 | 0.552 | 0.561 | 0.552 | 0.549 |
| TP + WTConv | NonInvasiveFetalECGThorax1 | 1.0 | 0.823 | 0.839 | 0.821 | 0.816 |
| TP + WTConv | NonInvasiveFetalECGThorax2 | 1.0 | 0.872 | 0.872 | 0.867 | 0.866 |
| TP + WTConv | Worms                      | 1.0 | 0.584 | 0.587 | 0.516 | 0.527 |
| TP + WTConv | WormsTwoClass              | 1.0 | 0.675 | 0.697 | 0.693 | 0.675 |
