# Supplementary material for: TimePoint: Accelerated Time Series Alignment via Self-Supervised Keypoint and Descriptor Learning
Source: arXiv:2505.23475 source file (2025-05-29)
Supplement: Supplementary file 4 [file all_ucr_tp20.pdf]

| TP         | Dataset                        | Keypoints Percentage | Accuracy | F1 Score | Precision | Recall |
|------------|--------------------------------|----------------------|----------|----------|-----------|--------|
| TP + Dense | SmoothSubspace                 | 0.2                  | 0.867    | 0.868    | 0.867     | 0.867  |
| TP + Dense | Chinatown                      | 0.2                  | 0.939    | 0.912    | 0.945     | 0.926  |
| TP + Dense | ItalyPowerDemand               | 0.2                  | 0.951    | 0.952    | 0.951     | 0.951  |
| TP + Dense | MelbournePedestrian            | 0.2                  | 0.1      | 0.01     | 0.1       | 0.018  |
| TP + Dense | Crop                           | 0.2                  | 0.684    | 0.666    | 0.684     | 0.672  |
| TP + Dense | SyntheticControl               | 0.2                  | 0.98     | 0.981    | 0.98      | 0.98   |
| TP + Dense | SonyAIBORobotSurface2          | 0.2                  | 0.877    | 0.868    | 0.883     | 0.873  |
| TP + Dense | SonyAIBORobotSurface1          | 0.2                  | 0.674    | 0.784    | 0.714     | 0.662  |
| TP + Dense | DistalPhalanxOutlineAgeGroup   | 0.2                  | 0.655    | 0.623    | 0.69      | 0.644  |
| TP + Dense | DistalPhalanxOutlineCorrect    | 0.2                  | 0.746    | 0.742    | 0.729     | 0.733  |
| TP + Dense | DistalPhalanxTW                | 0.2                  | 0.64     | 0.537    | 0.534     | 0.533  |
| TP + Dense | MiddlePhalanxOutlineAgeGroup   | 0.2                  | 0.468    | 0.44     | 0.451     | 0.432  |
| TP + Dense | MiddlePhalanxOutlineCorrect    | 0.2                  | 0.735    | 0.731    | 0.734     | 0.732  |
| TP + Dense | MiddlePhalanxTW                | 0.2                  | 0.532    | 0.426    | 0.432     | 0.425  |
| TP + Dense | PhalangesOutlinesCorrect       | 0.2                  | 0.767    | 0.756    | 0.745     | 0.75   |
| TP + Dense | ProximalPhalanxOutlineAgeGroup | 0.2                  | 0.785    | 0.704    | 0.694     | 0.697  |
| TP + Dense | ProximalPhalanxOutlineCorrect  | 0.2                  | 0.804    | 0.805    | 0.722     | 0.743  |
| TP + Dense | ProximalPhalanxTW              | 0.2                  | 0.712    | 0.478    | 0.466     | 0.466  |
| TP + Dense | TwoLeadECG                     | 0.2                  | 0.872    | 0.874    | 0.872     | 0.872  |
| TP + Dense | MoteStrain                     | 0.2                  | 0.869    | 0.872    | 0.865     | 0.867  |
| TP + Dense | ECG200                         | 0.2                  | 0.84     | 0.833    | 0.814     | 0.822  |
| TP + Dense | ElectricDevices                | 0.2                  | 0.611    | 0.551    | 0.497     | 0.51   |
| TP + Dense | MedicalImages                  | 0.2                  | 0.734    | 0.736    | 0.695     | 0.705  |

|            |             |     |       |       |       |       |
|------------|-------------|-----|-------|-------|-------|-------|
| TP + Dense | BME         | 0.2 | 0.907 | 0.927 | 0.907 | 0.907 |
| TP + Dense | CBF         | 0.2 | 0.997 | 0.997 | 0.997 | 0.997 |
| TP + Dense | SwedishLeaf | 0.2 | 0.904 | 0.912 | 0.907 | 0.906 |
| TP + Dense | TwoPatterns | 0.2 | 0.97  | 0.97  | 0.97  | 0.97  |
| TP + Dense | FaceAll     | 0.2 | 0.731 | 0.831 | 0.845 | 0.789 |
| TP + Dense | FacesUCR    | 0.2 | 0.909 | 0.911 | 0.884 | 0.891 |
| TP + Dense | ECGFiveDays | 0.2 | 0.714 | 0.745 | 0.715 | 0.706 |

| TP         | Dataset                  | Keypoints Percentage | Accuracy | F1 Score | Precision | Recall |
|------------|--------------------------|----------------------|----------|----------|-----------|--------|
| TP + Dense | ECG5000                  | 0.2                  | 0.925    | 0.647    | 0.546     | 0.569  |
| TP + Dense | Plane                    | 0.2                  | 1.0      | 1.0      | 1.0       | 1.0    |
| TP + Dense | PowerCons                | 0.2                  | 0.878    | 0.879    | 0.878     | 0.878  |
| TP + Dense | GunPoint                 | 0.2                  | 0.987    | 0.987    | 0.987     | 0.987  |
| TP + Dense | GunPointAgeSpan          | 0.2                  | 0.984    | 0.984    | 0.984     | 0.984  |
| TP + Dense | GunPointMaleVersusFemale | 0.2                  | 0.997    | 0.997    | 0.997     | 0.997  |
| TP + Dense | GunPointOldVersusYoung   | 0.2                  | 0.975    | 0.976    | 0.974     | 0.974  |
| TP + Dense | UMD                      | 0.2                  | 0.924    | 0.938    | 0.924     | 0.923  |
| TP + Dense | Wafer                    | 0.2                  | 0.982    | 0.974    | 0.931     | 0.951  |
| TP + Dense | ChlorineConcentration    | 0.2                  | 0.626    | 0.583    | 0.577     | 0.579  |
| TP + Dense | Adiac                    | 0.2                  | 0.65     | 0.659    | 0.649     | 0.628  |
| TP + Dense | Fungi                    | 0.2                  | 0.93     | 0.939    | 0.956     | 0.943  |
| TP + Dense | Wine                     | 0.2                  | 0.685    | 0.688    | 0.685     | 0.684  |
| TP + Dense | Strawberry               | 0.2                  | 0.946    | 0.937    | 0.948     | 0.942  |
| TP + Dense | ArrowHead                | 0.2                  | 0.817    | 0.831    | 0.834     | 0.818  |

|            |                      |     |       |       |       |       |
|------------|----------------------|-----|-------|-------|-------|-------|
| TP + Dense | InsectWingbeatSound  | 0.2 | 0.449 | 0.442 | 0.449 | 0.439 |
| TP + Dense | FiftyWords           | 0.2 | 0.763 | 0.718 | 0.643 | 0.644 |
| TP + Dense | WordSynonyms         | 0.2 | 0.715 | 0.68  | 0.597 | 0.607 |
| TP + Dense | Trace                | 0.2 | 1.0   | 1.0   | 1.0   | 1.0   |
| TP + Dense | ToeSegmentation1     | 0.2 | 0.833 | 0.861 | 0.826 | 0.827 |
| TP + Dense | Coffee               | 0.2 | 0.964 | 0.969 | 0.962 | 0.964 |
| TP + Dense | DodgerLoopDay        | 0.2 | 0.15  | 0.021 | 0.143 | 0.037 |
| TP + Dense | DodgerLoopGame       | 0.2 | 0.478 | 0.239 | 0.5   | 0.324 |
| TP + Dense | DodgerLoopWeekend    | 0.2 | 0.261 | 0.13  | 0.5   | 0.207 |
| TP + Dense | CricketX             | 0.2 | 0.713 | 0.726 | 0.714 | 0.716 |
| TP + Dense | CricketY             | 0.2 | 0.692 | 0.709 | 0.693 | 0.692 |
| TP + Dense | CricketZ             | 0.2 | 0.756 | 0.779 | 0.753 | 0.755 |
| TP + Dense | FreezerRegularTrain  | 0.2 | 0.909 | 0.909 | 0.909 | 0.909 |
| TP + Dense | FreezerSmallTrain    | 0.2 | 0.791 | 0.793 | 0.791 | 0.791 |
| TP + Dense | UWaveGestureLibraryX | 0.2 | 0.773 | 0.756 | 0.77  | 0.754 |

| TP         | Dataset              | Keypoints Percentage | Accuracy | F1 Score | Precision | Recall |
|------------|----------------------|----------------------|----------|----------|-----------|--------|
| TP + Dense | UWaveGestureLibraryY | 0.2                  | 0.681    | 0.683    | 0.681     | 0.678  |
| TP + Dense | UWaveGestureLibraryZ | 0.2                  | 0.702    | 0.689    | 0.704     | 0.687  |
| TP + Dense | Lightning7           | 0.2                  | 0.767    | 0.794    | 0.777     | 0.772  |
| TP + Dense | ToeSegmentation2     | 0.2                  | 0.938    | 0.883    | 0.93      | 0.904  |
| TP + Dense | DiatomSizeReduction  | 0.2                  | 0.961    | 0.971    | 0.909     | 0.929  |
| TP + Dense | FaceFour             | 0.2                  | 0.92     | 0.918    | 0.929     | 0.918  |
| TP + Dense | GestureMidAirD1      | 0.2                  | 0.038    | 0.001    | 0.038     | 0.003  |

|            |                       |     |       |       |       |       |
|------------|-----------------------|-----|-------|-------|-------|-------|
| TP + Dense | GestureMidAirD2       | 0.2 | 0.038 | 0.001 | 0.038 | 0.003 |
| TP + Dense | GestureMidAirD3       | 0.2 | 0.038 | 0.001 | 0.038 | 0.003 |
| TP + Dense | PickupGestureWiimoteZ | 0.2 | 0.1   | 0.01  | 0.1   | 0.018 |
| TP + Dense | AllGestureWiimoteX    | 0.2 | 0.1   | 0.01  | 0.1   | 0.018 |
| TP + Dense | AllGestureWiimoteY    | 0.2 | 0.1   | 0.01  | 0.1   | 0.018 |
| TP + Dense | AllGestureWiimoteZ    | 0.2 | 0.1   | 0.01  | 0.1   | 0.018 |
| TP + Dense | ShakeGestureWiimoteZ  | 0.2 | 0.1   | 0.01  | 0.1   | 0.018 |
| TP + Dense | Symbols               | 0.2 | 0.967 | 0.971 | 0.966 | 0.967 |
| TP + Dense | Yoga                  | 0.2 | 0.868 | 0.87  | 0.865 | 0.866 |
| TP + Dense | OSULeaf               | 0.2 | 0.798 | 0.819 | 0.802 | 0.803 |
| TP + Dense | Ham                   | 0.2 | 0.59  | 0.592 | 0.592 | 0.59  |
| TP + Dense | Meat                  | 0.2 | 0.833 | 0.852 | 0.833 | 0.835 |
| TP + Dense | GesturePebbleZ1       | 0.2 | 0.163 | 0.027 | 0.167 | 0.047 |
| TP + Dense | GesturePebbleZ2       | 0.2 | 0.152 | 0.025 | 0.167 | 0.044 |
| TP + Dense | Fish                  | 0.2 | 0.914 | 0.923 | 0.913 | 0.913 |
| TP + Dense | Beef                  | 0.2 | 0.7   | 0.763 | 0.7   | 0.703 |
| TP + Dense | FordA                 | 0.2 | 0.759 | 0.76  | 0.758 | 0.758 |
| TP + Dense | FordB                 | 0.2 | 0.709 | 0.709 | 0.709 | 0.709 |
| TP + Dense | ShapeletSim           | 0.2 | 0.661 | 0.665 | 0.661 | 0.659 |
| TP + Dense | BeetleFly             | 0.2 | 0.7   | 0.812 | 0.7   | 0.67  |
| TP + Dense | BirdChicken           | 0.2 | 0.75  | 0.753 | 0.75  | 0.749 |
| TP + Dense | Earthquakes           | 0.2 | 0.712 | 0.568 | 0.542 | 0.54  |
| TP + Dense | Herring               | 0.2 | 0.484 | 0.493 | 0.493 | 0.483 |

| TP          | Dataset                    | Keypoints Percentage | Accuracy | F1 Score | Precision | Recall |
|-------------|----------------------------|----------------------|----------|----------|-----------|--------|
| TP + Dense  | ShapesAll                  | 0.2                  | 0.86     | 0.879    | 0.86      | 0.857  |
| TP + Dense  | OliveOil                   | 0.2                  | 0.6      | 0.624    | 0.558     | 0.578  |
| TP + Dense  | Car                        | 0.2                  | 0.85     | 0.89     | 0.833     | 0.822  |
| TP + Dense  | InsectEPGRegularTrain      | 0.2                  | 0.916    | 0.904    | 0.899     | 0.901  |
| TP + Dense  | InsectEPGSmallTrain        | 0.2                  | 0.819    | 0.792    | 0.818     | 0.797  |
| TP + Dense  | Lightning2                 | 0.2                  | 0.82     | 0.83     | 0.812     | 0.815  |
| TP + Dense  | Computers                  | 0.2                  | 0.58     | 0.581    | 0.58      | 0.579  |
| TP + Dense  | LargeKitchenAppliances     | 0.2                  | 0.784    | 0.791    | 0.784     | 0.784  |
| TP + Dense  | RefrigerationDevices       | 0.2                  | 0.496    | 0.506    | 0.496     | 0.499  |
| TP + Dense  | ScreenType                 | 0.2                  | 0.416    | 0.423    | 0.416     | 0.414  |
| TP + Dense  | SmallKitchenAppliances     | 0.2                  | 0.664    | 0.665    | 0.664     | 0.661  |
| TP + Dense  | NonInvasiveFetalECGThorax1 | 0.2                  | 0.717    | 0.745    | 0.715     | 0.708  |
| TP + Dense  | NonInvasiveFetalECGThorax2 | 0.2                  | 0.807    | 0.808    | 0.802     | 0.797  |
| TP + Dense  | Worms                      | 0.2                  | 0.597    | 0.635    | 0.574     | 0.586  |
| TP + Dense  | WormsTwoClass              | 0.2                  | 0.714    | 0.71     | 0.712     | 0.71   |
| TP + WTConv | SmoothSubspace             | 0.2                  | 0.793    | 0.801    | 0.793     | 0.787  |
| TP + WTConv | Chinatown                  | 0.2                  | 0.924    | 0.895    | 0.928     | 0.909  |
| TP + WTConv | ItalyPowerDemand           | 0.2                  | 0.934    | 0.934    | 0.934     | 0.934  |
| TP + WTConv | MelbournePedestrian        | 0.2                  | 0.1      | 0.01     | 0.1       | 0.018  |
| TP + WTConv | Crop                       | 0.2                  | 0.693    | 0.677    | 0.693     | 0.681  |
| TP + WTConv | SyntheticControl           | 0.2                  | 0.977    | 0.977    | 0.977     | 0.977  |
| TP + WTConv | SonyAIBORobotSurface2      | 0.2                  | 0.886    | 0.882    | 0.874     | 0.878  |
| TP + WTConv | SonyAIBORobotSurface1      | 0.2                  | 0.764    | 0.822    | 0.793     | 0.762  |

|             |                              |     |       |       |       |       |
|-------------|------------------------------|-----|-------|-------|-------|-------|
| TP + WTConv | DistalPhalanxOutlineAgeGroup | 0.2 | 0.619 | 0.559 | 0.594 | 0.567 |
| TP + WTConv | DistalPhalanxOutlineCorrect  | 0.2 | 0.692 | 0.684 | 0.671 | 0.674 |
| TP + WTConv | DistalPhalanxTW              | 0.2 | 0.59  | 0.446 | 0.449 | 0.445 |
| TP + WTConv | MiddlePhalanxOutlineAgeGroup | 0.2 | 0.39  | 0.37  | 0.38  | 0.362 |
| TP + WTConv | MiddlePhalanxOutlineCorrect  | 0.2 | 0.729 | 0.723 | 0.722 | 0.722 |
| TP + WTConv | MiddlePhalanxTW              | 0.2 | 0.474 | 0.385 | 0.389 | 0.38  |
| TP + WTConv | PhalangesOutlinesCorrect     | 0.2 | 0.727 | 0.712 | 0.712 | 0.712 |

| TP          | Dataset                        | Keypoints Percentage | Accuracy | F1 Score | Precision | Recall |
|-------------|--------------------------------|----------------------|----------|----------|-----------|--------|
| TP + WTConv | ProximalPhalanxOutlineAgeGroup | 0.2                  | 0.805    | 0.727    | 0.774     | 0.744  |
| TP + WTConv | ProximalPhalanxOutlineCorrect  | 0.2                  | 0.821    | 0.822    | 0.75      | 0.77   |
| TP + WTConv | ProximalPhalanxTW              | 0.2                  | 0.693    | 0.394    | 0.389     | 0.389  |
| TP + WTConv | TwoLeadECG                     | 0.2                  | 0.816    | 0.819    | 0.816     | 0.815  |
| TP + WTConv | MoteStrain                     | 0.2                  | 0.861    | 0.864    | 0.857     | 0.859  |
| TP + WTConv | ECG200                         | 0.2                  | 0.82     | 0.814    | 0.786     | 0.796  |
| TP + WTConv | ElectricDevices                | 0.2                  | 0.607    | 0.554    | 0.517     | 0.526  |
| TP + WTConv | MedicalImages                  | 0.2                  | 0.714    | 0.714    | 0.678     | 0.688  |
| TP + WTConv | BME                            | 0.2                  | 0.94     | 0.949    | 0.94      | 0.941  |
| TP + WTConv | CBF                            | 0.2                  | 0.99     | 0.99     | 0.99      | 0.99   |
| TP + WTConv | SwedishLeaf                    | 0.2                  | 0.904    | 0.911    | 0.908     | 0.905  |
| TP + WTConv | TwoPatterns                    | 0.2                  | 0.771    | 0.771    | 0.771     | 0.771  |
| TP + WTConv | FaceAll                        | 0.2                  | 0.717    | 0.777    | 0.819     | 0.745  |
| TP + WTConv | FacesUCR                       | 0.2                  | 0.84     | 0.842    | 0.8       | 0.812  |
| TP + WTConv | ECGFiveDays                    | 0.2                  | 0.897    | 0.905    | 0.897     | 0.896  |

|             |                          |     |       |       |       |       |
|-------------|--------------------------|-----|-------|-------|-------|-------|
| TP + WTConv | ECG5000                  | 0.2 | 0.924 | 0.679 | 0.558 | 0.577 |
| TP + WTConv | Plane                    | 0.2 | 0.99  | 0.991 | 0.991 | 0.991 |
| TP + WTConv | PowerCons                | 0.2 | 0.906 | 0.921 | 0.906 | 0.905 |
| TP + WTConv | GunPoint                 | 0.2 | 0.993 | 0.994 | 0.993 | 0.993 |
| TP + WTConv | GunPointAgeSpan          | 0.2 | 0.975 | 0.975 | 0.975 | 0.975 |
| TP + WTConv | GunPointMaleVersusFemale | 0.2 | 1.0   | 1.0   | 1.0   | 1.0   |
| TP + WTConv | GunPointOldVersusYoung   | 0.2 | 0.971 | 0.974 | 0.97  | 0.971 |
| TP + WTConv | UMD                      | 0.2 | 0.889 | 0.887 | 0.889 | 0.888 |
| TP + WTConv | Wafer                    | 0.2 | 0.993 | 0.982 | 0.979 | 0.981 |
| TP + WTConv | ChlorineConcentration    | 0.2 | 0.624 | 0.582 | 0.573 | 0.577 |
| TP + WTConv | Adiac                    | 0.2 | 0.678 | 0.695 | 0.679 | 0.661 |
| TP + WTConv | Fungi                    | 0.2 | 0.995 | 0.995 | 0.997 | 0.996 |
| TP + WTConv | Wine                     | 0.2 | 0.722 | 0.723 | 0.722 | 0.722 |
| TP + WTConv | Strawberry               | 0.2 | 0.951 | 0.941 | 0.957 | 0.948 |
| TP + WTConv | ArrowHead                | 0.2 | 0.851 | 0.851 | 0.857 | 0.851 |

| TP          | Dataset             | Keypoints Percentage | Accuracy | F1 Score | Precision | Recall |
|-------------|---------------------|----------------------|----------|----------|-----------|--------|
| TP + WTConv | InsectWingbeatSound | 0.2                  | 0.534    | 0.529    | 0.534     | 0.528  |
| TP + WTConv | FiftyWords          | 0.2                  | 0.76     | 0.647    | 0.66      | 0.631  |
| TP + WTConv | WordSynonyms        | 0.2                  | 0.721    | 0.644    | 0.581     | 0.589  |
| TP + WTConv | Trace               | 0.2                  | 0.99     | 0.988    | 0.991     | 0.989  |
| TP + WTConv | ToeSegmentation1    | 0.2                  | 0.838    | 0.837    | 0.838     | 0.837  |
| TP + WTConv | Coffee              | 0.2                  | 1.0      | 1.0      | 1.0       | 1.0    |
| TP + WTConv | DodgerLoopDay       | 0.2                  | 0.15     | 0.021    | 0.143     | 0.037  |

|            |                       |     |       |       |       |       |
|------------|-----------------------|-----|-------|-------|-------|-------|
| TP + WTCnv | DodgerLoopGame        | 0.2 | 0.478 | 0.239 | 0.5   | 0.324 |
| TP + WTCnv | DodgerLoopWeekend     | 0.2 | 0.261 | 0.13  | 0.5   | 0.207 |
| TP + WTCnv | CricketX              | 0.2 | 0.703 | 0.727 | 0.707 | 0.707 |
| TP + WTCnv | CricketY              | 0.2 | 0.731 | 0.751 | 0.73  | 0.734 |
| TP + WTCnv | CricketZ              | 0.2 | 0.723 | 0.733 | 0.718 | 0.718 |
| TP + WTCnv | FreezerRegularTrain   | 0.2 | 0.927 | 0.927 | 0.927 | 0.927 |
| TP + WTCnv | FreezerSmallTrain     | 0.2 | 0.793 | 0.794 | 0.793 | 0.792 |
| TP + WTCnv | UWaveGestureLibraryX  | 0.2 | 0.791 | 0.778 | 0.789 | 0.781 |
| TP + WTCnv | UWaveGestureLibraryY  | 0.2 | 0.73  | 0.726 | 0.731 | 0.725 |
| TP + WTCnv | UWaveGestureLibraryZ  | 0.2 | 0.728 | 0.716 | 0.73  | 0.717 |
| TP + WTCnv | Lightning7            | 0.2 | 0.74  | 0.798 | 0.73  | 0.735 |
| TP + WTCnv | ToeSegmentation2      | 0.2 | 0.885 | 0.803 | 0.881 | 0.831 |
| TP + WTCnv | DiatomSizeReduction   | 0.2 | 0.958 | 0.968 | 0.902 | 0.922 |
| TP + WTCnv | FaceFour              | 0.2 | 0.932 | 0.929 | 0.939 | 0.93  |
| TP + WTCnv | GestureMidAirD1       | 0.2 | 0.038 | 0.001 | 0.038 | 0.003 |
| TP + WTCnv | GestureMidAirD2       | 0.2 | 0.038 | 0.001 | 0.038 | 0.003 |
| TP + WTCnv | GestureMidAirD3       | 0.2 | 0.038 | 0.001 | 0.038 | 0.003 |
| TP + WTCnv | PickupGestureWiimoteZ | 0.2 | 0.1   | 0.01  | 0.1   | 0.018 |
| TP + WTCnv | AllGestureWiimoteX    | 0.2 | 0.1   | 0.01  | 0.1   | 0.018 |
| TP + WTCnv | AllGestureWiimoteY    | 0.2 | 0.1   | 0.01  | 0.1   | 0.018 |
| TP + WTCnv | AllGestureWiimoteZ    | 0.2 | 0.1   | 0.01  | 0.1   | 0.018 |
| TP + WTCnv | ShakeGestureWiimoteZ  | 0.2 | 0.1   | 0.01  | 0.1   | 0.018 |
| TP + WTCnv | Symbols               | 0.2 | 0.955 | 0.959 | 0.953 | 0.955 |



| TP          | Dataset                | Keypoints Percentage | Accuracy | F1 Score | Precision | Recall |
|-------------|------------------------|----------------------|----------|----------|-----------|--------|
| TP + WTConv | Yoga                   | 0.2                  | 0.866    | 0.869    | 0.863     | 0.865  |
| TP + WTConv | OSULeaf                | 0.2                  | 0.793    | 0.83     | 0.802     | 0.802  |
| TP + WTConv | Ham                    | 0.2                  | 0.533    | 0.533    | 0.533     | 0.533  |
| TP + WTConv | Meat                   | 0.2                  | 0.9      | 0.909    | 0.9       | 0.9    |
| TP + WTConv | GesturePebbleZ1        | 0.2                  | 0.163    | 0.027    | 0.167     | 0.047  |
| TP + WTConv | GesturePebbleZ2        | 0.2                  | 0.152    | 0.025    | 0.167     | 0.044  |
| TP + WTConv | Fish                   | 0.2                  | 0.903    | 0.903    | 0.904     | 0.901  |
| TP + WTConv | Beef                   | 0.2                  | 0.767    | 0.779    | 0.767     | 0.768  |
| TP + WTConv | FordA                  | 0.2                  | 0.775    | 0.786    | 0.772     | 0.771  |
| TP + WTConv | FordB                  | 0.2                  | 0.64     | 0.642    | 0.64      | 0.638  |
| TP + WTConv | ShapeletSim            | 0.2                  | 0.644    | 0.648    | 0.644     | 0.642  |
| TP + WTConv | BeetleFly              | 0.2                  | 0.85     | 0.885    | 0.85      | 0.847  |
| TP + WTConv | BirdChicken            | 0.2                  | 0.75     | 0.775    | 0.75      | 0.744  |
| TP + WTConv | Earthquakes            | 0.2                  | 0.662    | 0.499    | 0.499     | 0.494  |
| TP + WTConv | Herring                | 0.2                  | 0.547    | 0.544    | 0.546     | 0.541  |
| TP + WTConv | ShapesAll              | 0.2                  | 0.873    | 0.893    | 0.873     | 0.868  |
| TP + WTConv | OliveOil               | 0.2                  | 0.7      | 0.616    | 0.586     | 0.592  |
| TP + WTConv | Car                    | 0.2                  | 0.85     | 0.847    | 0.848     | 0.847  |
| TP + WTConv | InsectEPGRegularTrain  | 0.2                  | 0.932    | 0.921    | 0.907     | 0.914  |
| TP + WTConv | InsectEPGSmallTrain    | 0.2                  | 0.795    | 0.772    | 0.806     | 0.778  |
| TP + WTConv | Lightning2             | 0.2                  | 0.869    | 0.868    | 0.868     | 0.868  |
| TP + WTConv | Computers              | 0.2                  | 0.676    | 0.676    | 0.676     | 0.676  |
| TP + WTConv | LargeKitchenAppliances | 0.2                  | 0.744    | 0.743    | 0.744     | 0.743  |

|             |                            |     |       |       |       |       |
|-------------|----------------------------|-----|-------|-------|-------|-------|
| TP + WTConv | RefrigerationDevices       | 0.2 | 0.491 | 0.497 | 0.491 | 0.491 |
| TP + WTConv | ScreenType                 | 0.2 | 0.419 | 0.423 | 0.419 | 0.419 |
| TP + WTConv | SmallKitchenAppliances     | 0.2 | 0.579 | 0.594 | 0.579 | 0.577 |
| TP + WTConv | NonInvasiveFetalECGThorax1 | 0.2 | 0.798 | 0.815 | 0.797 | 0.791 |
| TP + WTConv | NonInvasiveFetalECGThorax2 | 0.2 | 0.867 | 0.87  | 0.863 | 0.864 |
| TP + WTConv | Worms                      | 0.2 | 0.584 | 0.621 | 0.521 | 0.536 |
| TP + WTConv | WormsTwoClass              | 0.2 | 0.636 | 0.668 | 0.659 | 0.635 |
