# Supplementary material for: TimePoint: Accelerated Time Series Alignment via Self-Supervised Keypoint and Descriptor Learning
Source: arXiv:2505.23475 source file (2025-05-29)
Supplement: Supplementary file 5 [file all_ucr_tp50.pdf]

| TP         | Dataset                        | Keypoints Percentage | Accuracy | F1 Score | Precision | Recall |
|------------|--------------------------------|----------------------|----------|----------|-----------|--------|
| TP + Dense | SmoothSubspace                 | 0.5                  | 0.873    | 0.88     | 0.873     | 0.874  |
| TP + Dense | Chinatown                      | 0.5                  | 0.924    | 0.893    | 0.935     | 0.91   |
| TP + Dense | ItalyPowerDemand               | 0.5                  | 0.96     | 0.96     | 0.96      | 0.96   |
| TP + Dense | MelbournePedestrian            | 0.5                  | 0.1      | 0.01     | 0.1       | 0.018  |
| TP + Dense | Crop                           | 0.5                  | 0.683    | 0.668    | 0.683     | 0.672  |
| TP + Dense | SyntheticControl               | 0.5                  | 0.973    | 0.975    | 0.973     | 0.973  |
| TP + Dense | SonyAIBORobotSurface2          | 0.5                  | 0.875    | 0.867    | 0.885     | 0.872  |
| TP + Dense | SonyAIBORobotSurface1          | 0.5                  | 0.714    | 0.8      | 0.749     | 0.708  |
| TP + Dense | DistalPhalanxOutlineAgeGroup   | 0.5                  | 0.626    | 0.597    | 0.666     | 0.617  |
| TP + Dense | DistalPhalanxOutlineCorrect    | 0.5                  | 0.75     | 0.749    | 0.73      | 0.734  |
| TP + Dense | DistalPhalanxTW                | 0.5                  | 0.676    | 0.583    | 0.573     | 0.574  |
| TP + Dense | MiddlePhalanxOutlineAgeGroup   | 0.5                  | 0.442    | 0.396    | 0.405     | 0.397  |
| TP + Dense | MiddlePhalanxOutlineCorrect    | 0.5                  | 0.725    | 0.721    | 0.724     | 0.722  |
| TP + Dense | MiddlePhalanxTW                | 0.5                  | 0.539    | 0.419    | 0.415     | 0.414  |
| TP + Dense | PhalangesOutlinesCorrect       | 0.5                  | 0.745    | 0.732    | 0.72      | 0.724  |
| TP + Dense | ProximalPhalanxOutlineAgeGroup | 0.5                  | 0.815    | 0.725    | 0.749     | 0.733  |
| TP + Dense | ProximalPhalanxOutlineCorrect  | 0.5                  | 0.835    | 0.852    | 0.76      | 0.784  |
| TP + Dense | ProximalPhalanxTW              | 0.5                  | 0.737    | 0.48     | 0.462     | 0.466  |
| TP + Dense | TwoLeadECG                     | 0.5                  | 0.839    | 0.843    | 0.839     | 0.839  |
| TP + Dense | MoteStrain                     | 0.5                  | 0.865    | 0.869    | 0.861     | 0.863  |
| TP + Dense | ECG200                         | 0.5                  | 0.87     | 0.878    | 0.838     | 0.852  |
| TP + Dense | ElectricDevices                | 0.5                  | 0.614    | 0.544    | 0.501     | 0.512  |
| TP + Dense | MedicalImages                  | 0.5                  | 0.717    | 0.719    | 0.678     | 0.69   |

|            |             |     |       |       |       |       |
|------------|-------------|-----|-------|-------|-------|-------|
| TP + Dense | BME         | 0.5 | 0.833 | 0.889 | 0.833 | 0.827 |
| TP + Dense | CBF         | 0.5 | 0.988 | 0.988 | 0.988 | 0.988 |
| TP + Dense | SwedishLeaf | 0.5 | 0.893 | 0.897 | 0.896 | 0.894 |
| TP + Dense | TwoPatterns | 0.5 | 0.877 | 0.878 | 0.877 | 0.877 |
| TP + Dense | FaceAll     | 0.5 | 0.721 | 0.816 | 0.838 | 0.778 |
| TP + Dense | FacesUCR    | 0.5 | 0.895 | 0.892 | 0.869 | 0.876 |
| TP + Dense | ECGFiveDays | 0.5 | 0.758 | 0.782 | 0.759 | 0.754 |

| TP         | Dataset                  | Keypoints Percentage | Accuracy | F1 Score | Precision | Recall |
|------------|--------------------------|----------------------|----------|----------|-----------|--------|
| TP + Dense | ECG5000                  | 0.5                  | 0.923    | 0.671    | 0.552     | 0.577  |
| TP + Dense | Plane                    | 0.5                  | 1.0      | 1.0      | 1.0       | 1.0    |
| TP + Dense | PowerCons                | 0.5                  | 0.872    | 0.872    | 0.872     | 0.872  |
| TP + Dense | GunPoint                 | 0.5                  | 0.987    | 0.987    | 0.986     | 0.987  |
| TP + Dense | GunPointAgeSpan          | 0.5                  | 0.978    | 0.979    | 0.978     | 0.978  |
| TP + Dense | GunPointMaleVersusFemale | 0.5                  | 0.997    | 0.997    | 0.997     | 0.997  |
| TP + Dense | GunPointOldVersusYoung   | 0.5                  | 0.959    | 0.961    | 0.957     | 0.958  |
| TP + Dense | UMD                      | 0.5                  | 0.91     | 0.92     | 0.91      | 0.91   |
| TP + Dense | Wafer                    | 0.5                  | 0.982    | 0.975    | 0.931     | 0.952  |
| TP + Dense | ChlorineConcentration    | 0.5                  | 0.626    | 0.582    | 0.575     | 0.577  |
| TP + Dense | Adiac                    | 0.5                  | 0.683    | 0.693    | 0.675     | 0.661  |
| TP + Dense | Fungi                    | 0.5                  | 0.866    | 0.909    | 0.898     | 0.888  |
| TP + Dense | Wine                     | 0.5                  | 0.574    | 0.574    | 0.574     | 0.574  |
| TP + Dense | Strawberry               | 0.5                  | 0.943    | 0.934    | 0.944     | 0.939  |
| TP + Dense | ArrowHead                | 0.5                  | 0.737    | 0.761    | 0.763     | 0.732  |

|            |                      |     |       |       |       |       |
|------------|----------------------|-----|-------|-------|-------|-------|
| TP + Dense | InsectWingbeatSound  | 0.5 | 0.433 | 0.425 | 0.433 | 0.425 |
| TP + Dense | FiftyWords           | 0.5 | 0.734 | 0.695 | 0.621 | 0.62  |
| TP + Dense | WordSynonyms         | 0.5 | 0.691 | 0.615 | 0.56  | 0.568 |
| TP + Dense | Trace                | 0.5 | 1.0   | 1.0   | 1.0   | 1.0   |
| TP + Dense | ToeSegmentation1     | 0.5 | 0.833 | 0.857 | 0.826 | 0.828 |
| TP + Dense | Coffee               | 0.5 | 0.964 | 0.969 | 0.962 | 0.964 |
| TP + Dense | DodgerLoopDay        | 0.5 | 0.15  | 0.021 | 0.143 | 0.037 |
| TP + Dense | DodgerLoopGame       | 0.5 | 0.478 | 0.239 | 0.5   | 0.324 |
| TP + Dense | DodgerLoopWeekend    | 0.5 | 0.261 | 0.13  | 0.5   | 0.207 |
| TP + Dense | CricketX             | 0.5 | 0.608 | 0.629 | 0.611 | 0.611 |
| TP + Dense | CricketY             | 0.5 | 0.569 | 0.59  | 0.568 | 0.559 |
| TP + Dense | CricketZ             | 0.5 | 0.585 | 0.637 | 0.586 | 0.585 |
| TP + Dense | FreezerRegularTrain  | 0.5 | 0.867 | 0.868 | 0.867 | 0.867 |
| TP + Dense | FreezerSmallTrain    | 0.5 | 0.77  | 0.772 | 0.77  | 0.77  |
| TP + Dense | UWaveGestureLibraryX | 0.5 | 0.768 | 0.75  | 0.765 | 0.749 |

| TP         | Dataset              | Keypoints Percentage | Accuracy | F1 Score | Precision | Recall |
|------------|----------------------|----------------------|----------|----------|-----------|--------|
| TP + Dense | UWaveGestureLibraryY | 0.5                  | 0.676    | 0.678    | 0.676     | 0.673  |
| TP + Dense | UWaveGestureLibraryZ | 0.5                  | 0.673    | 0.664    | 0.675     | 0.659  |
| TP + Dense | Lightning7           | 0.5                  | 0.726    | 0.73     | 0.755     | 0.73   |
| TP + Dense | ToeSegmentation2     | 0.5                  | 0.915    | 0.845    | 0.916     | 0.873  |
| TP + Dense | DiatomSizeReduction  | 0.5                  | 0.974    | 0.98     | 0.939     | 0.955  |
| TP + Dense | FaceFour             | 0.5                  | 0.875    | 0.877    | 0.889     | 0.871  |
| TP + Dense | GestureMidAirD1      | 0.5                  | 0.038    | 0.001    | 0.038     | 0.003  |

|            |                       |     |       |       |       |       |
|------------|-----------------------|-----|-------|-------|-------|-------|
| TP + Dense | GestureMidAirD2       | 0.5 | 0.038 | 0.001 | 0.038 | 0.003 |
| TP + Dense | GestureMidAirD3       | 0.5 | 0.038 | 0.001 | 0.038 | 0.003 |
| TP + Dense | PickupGestureWiimoteZ | 0.5 | 0.1   | 0.01  | 0.1   | 0.018 |
| TP + Dense | AllGestureWiimoteX    | 0.5 | 0.1   | 0.01  | 0.1   | 0.018 |
| TP + Dense | AllGestureWiimoteY    | 0.5 | 0.1   | 0.01  | 0.1   | 0.018 |
| TP + Dense | AllGestureWiimoteZ    | 0.5 | 0.1   | 0.01  | 0.1   | 0.018 |
| TP + Dense | ShakeGestureWiimoteZ  | 0.5 | 0.1   | 0.01  | 0.1   | 0.018 |
| TP + Dense | Symbols               | 0.5 | 0.968 | 0.97  | 0.968 | 0.968 |
| TP + Dense | Yoga                  | 0.5 | 0.863 | 0.865 | 0.861 | 0.862 |
| TP + Dense | OSULeaf               | 0.5 | 0.736 | 0.763 | 0.757 | 0.747 |
| TP + Dense | Ham                   | 0.5 | 0.495 | 0.493 | 0.493 | 0.492 |
| TP + Dense | Meat                  | 0.5 | 0.8   | 0.829 | 0.8   | 0.799 |
| TP + Dense | GesturePebbleZ1       | 0.5 | 0.163 | 0.027 | 0.167 | 0.047 |
| TP + Dense | GesturePebbleZ2       | 0.5 | 0.152 | 0.025 | 0.167 | 0.044 |
| TP + Dense | Fish                  | 0.5 | 0.874 | 0.872 | 0.874 | 0.871 |
| TP + Dense | Beef                  | 0.5 | 0.633 | 0.678 | 0.633 | 0.631 |
| TP + Dense | FordA                 | 0.5 | 0.764 | 0.765 | 0.763 | 0.764 |
| TP + Dense | FordB                 | 0.5 | 0.691 | 0.692 | 0.691 | 0.691 |
| TP + Dense | ShapeletSim           | 0.5 | 0.589 | 0.593 | 0.589 | 0.585 |
| TP + Dense | BeetleFly             | 0.5 | 0.65  | 0.794 | 0.65  | 0.601 |
| TP + Dense | BirdChicken           | 0.5 | 0.75  | 0.753 | 0.75  | 0.749 |
| TP + Dense | Earthquakes           | 0.5 | 0.727 | 0.62  | 0.599 | 0.606 |
| TP + Dense | Herring               | 0.5 | 0.578 | 0.575 | 0.578 | 0.573 |

| TP          | Dataset                    | Keypoints Percentage | Accuracy | F1 Score | Precision | Recall |
|-------------|----------------------------|----------------------|----------|----------|-----------|--------|
| TP + Dense  | ShapesAll                  | 0.5                  | 0.838    | 0.856    | 0.838     | 0.833  |
| TP + Dense  | OliveOil                   | 0.5                  | 0.767    | 0.828    | 0.686     | 0.698  |
| TP + Dense  | Car                        | 0.5                  | 0.817    | 0.816    | 0.82      | 0.809  |
| TP + Dense  | InsectEPGRegularTrain      | 0.5                  | 0.871    | 0.844    | 0.849     | 0.846  |
| TP + Dense  | InsectEPGSmallTrain        | 0.5                  | 0.791    | 0.756    | 0.76      | 0.756  |
| TP + Dense  | Lightning2                 | 0.5                  | 0.77     | 0.77     | 0.766     | 0.767  |
| TP + Dense  | Computers                  | 0.5                  | 0.632    | 0.632    | 0.632     | 0.632  |
| TP + Dense  | LargeKitchenAppliances     | 0.5                  | 0.755    | 0.759    | 0.755     | 0.753  |
| TP + Dense  | RefrigerationDevices       | 0.5                  | 0.475    | 0.485    | 0.475     | 0.478  |
| TP + Dense  | ScreenType                 | 0.5                  | 0.411    | 0.414    | 0.411     | 0.409  |
| TP + Dense  | SmallKitchenAppliances     | 0.5                  | 0.629    | 0.642    | 0.629     | 0.622  |
| TP + Dense  | NonInvasiveFetalECGThorax1 | 0.5                  | 0.642    | 0.675    | 0.64      | 0.629  |
| TP + Dense  | NonInvasiveFetalECGThorax2 | 0.5                  | 0.758    | 0.755    | 0.751     | 0.745  |
| TP + Dense  | Worms                      | 0.5                  | 0.597    | 0.633    | 0.564     | 0.557  |
| TP + Dense  | WormsTwoClass              | 0.5                  | 0.714    | 0.712    | 0.716     | 0.712  |
| TP + WTConv | SmoothSubspace             | 0.5                  | 0.807    | 0.818    | 0.807     | 0.801  |
| TP + WTConv | Chinatown                  | 0.5                  | 0.915    | 0.883    | 0.925     | 0.9    |
| TP + WTConv | ItalyPowerDemand           | 0.5                  | 0.957    | 0.957    | 0.957     | 0.957  |
| TP + WTConv | MelbournePedestrian        | 0.5                  | 0.1      | 0.01     | 0.1       | 0.018  |
| TP + WTConv | Crop                       | 0.5                  | 0.682    | 0.666    | 0.682     | 0.671  |
| TP + WTConv | SyntheticControl           | 0.5                  | 0.967    | 0.968    | 0.967     | 0.967  |
| TP + WTConv | SonyAIBORobotSurface2      | 0.5                  | 0.89     | 0.883    | 0.885     | 0.884  |
| TP + WTConv | SonyAIBORobotSurface1      | 0.5                  | 0.76     | 0.821    | 0.79      | 0.758  |

|             |                              |     |       |       |       |       |
|-------------|------------------------------|-----|-------|-------|-------|-------|
| TP + WTConv | DistalPhalanxOutlineAgeGroup | 0.5 | 0.633 | 0.588 | 0.655 | 0.605 |
| TP + WTConv | DistalPhalanxOutlineCorrect  | 0.5 | 0.699 | 0.694 | 0.675 | 0.678 |
| TP + WTConv | DistalPhalanxTW              | 0.5 | 0.583 | 0.44  | 0.454 | 0.445 |
| TP + WTConv | MiddlePhalanxOutlineAgeGroup | 0.5 | 0.461 | 0.447 | 0.461 | 0.435 |
| TP + WTConv | MiddlePhalanxOutlineCorrect  | 0.5 | 0.694 | 0.69  | 0.692 | 0.69  |
| TP + WTConv | MiddlePhalanxTW              | 0.5 | 0.539 | 0.429 | 0.425 | 0.422 |
| TP + WTConv | PhalangesOutlinesCorrect     | 0.5 | 0.748 | 0.735 | 0.728 | 0.731 |

| TP          | Dataset                        | Keypoints Percentage | Accuracy | F1 Score | Precision | Recall |
|-------------|--------------------------------|----------------------|----------|----------|-----------|--------|
| TP + WTConv | ProximalPhalanxOutlineAgeGroup | 0.5                  | 0.805    | 0.717    | 0.757     | 0.729  |
| TP + WTConv | ProximalPhalanxOutlineCorrect  | 0.5                  | 0.825    | 0.815    | 0.764     | 0.781  |
| TP + WTConv | ProximalPhalanxTW              | 0.5                  | 0.712    | 0.442    | 0.484     | 0.443  |
| TP + WTConv | TwoLeadECG                     | 0.5                  | 0.801    | 0.806    | 0.801     | 0.8    |
| TP + WTConv | MoteStrain                     | 0.5                  | 0.852    | 0.856    | 0.847     | 0.85   |
| TP + WTConv | ECG200                         | 0.5                  | 0.82     | 0.814    | 0.786     | 0.796  |
| TP + WTConv | ElectricDevices                | 0.5                  | 0.616    | 0.556    | 0.523     | 0.53   |
| TP + WTConv | MedicalImages                  | 0.5                  | 0.729    | 0.703    | 0.681     | 0.681  |
| TP + WTConv | BME                            | 0.5                  | 0.893    | 0.919    | 0.893     | 0.891  |
| TP + WTConv | CBF                            | 0.5                  | 0.94     | 0.943    | 0.94      | 0.94   |
| TP + WTConv | SwedishLeaf                    | 0.5                  | 0.888    | 0.898    | 0.892     | 0.89   |
| TP + WTConv | TwoPatterns                    | 0.5                  | 0.687    | 0.687    | 0.687     | 0.687  |
| TP + WTConv | FaceAll                        | 0.5                  | 0.72     | 0.781    | 0.828     | 0.745  |
| TP + WTConv | FacesUCR                       | 0.5                  | 0.802    | 0.81     | 0.764     | 0.777  |
| TP + WTConv | ECGFiveDays                    | 0.5                  | 0.942    | 0.943    | 0.942     | 0.942  |

|             |                          |     |       |       |       |       |
|-------------|--------------------------|-----|-------|-------|-------|-------|
| TP + WTConv | ECG5000                  | 0.5 | 0.921 | 0.767 | 0.56  | 0.584 |
| TP + WTConv | Plane                    | 0.5 | 1.0   | 1.0   | 1.0   | 1.0   |
| TP + WTConv | PowerCons                | 0.5 | 0.878 | 0.894 | 0.878 | 0.877 |
| TP + WTConv | GunPoint                 | 0.5 | 0.973 | 0.975 | 0.973 | 0.973 |
| TP + WTConv | GunPointAgeSpan          | 0.5 | 0.972 | 0.972 | 0.972 | 0.972 |
| TP + WTConv | GunPointMaleVersusFemale | 0.5 | 0.997 | 0.997 | 0.997 | 0.997 |
| TP + WTConv | GunPointOldVersusYoung   | 0.5 | 0.959 | 0.961 | 0.957 | 0.958 |
| TP + WTConv | UMD                      | 0.5 | 0.84  | 0.84  | 0.84  | 0.838 |
| TP + WTConv | Wafer                    | 0.5 | 0.989 | 0.98  | 0.965 | 0.972 |
| TP + WTConv | ChlorineConcentration    | 0.5 | 0.648 | 0.607 | 0.599 | 0.602 |
| TP + WTConv | Adiac                    | 0.5 | 0.734 | 0.747 | 0.73  | 0.717 |
| TP + WTConv | Fungi                    | 0.5 | 0.925 | 0.925 | 0.924 | 0.911 |
| TP + WTConv | Wine                     | 0.5 | 0.741 | 0.742 | 0.741 | 0.74  |
| TP + WTConv | Strawberry               | 0.5 | 0.943 | 0.932 | 0.949 | 0.939 |
| TP + WTConv | ArrowHead                | 0.5 | 0.874 | 0.874 | 0.881 | 0.874 |

| TP          | Dataset             | Keypoints Percentage | Accuracy | F1 Score | Precision | Recall |
|-------------|---------------------|----------------------|----------|----------|-----------|--------|
| TP + WTConv | InsectWingbeatSound | 0.5                  | 0.504    | 0.499    | 0.504     | 0.499  |
| TP + WTConv | FiftyWords          | 0.5                  | 0.736    | 0.645    | 0.607     | 0.592  |
| TP + WTConv | WordSynonyms        | 0.5                  | 0.694    | 0.598    | 0.545     | 0.551  |
| TP + WTConv | Trace               | 0.5                  | 0.99     | 0.988    | 0.991     | 0.989  |
| TP + WTConv | ToeSegmentation1    | 0.5                  | 0.855    | 0.858    | 0.853     | 0.854  |
| TP + WTConv | Coffee              | 0.5                  | 1.0      | 1.0      | 1.0       | 1.0    |
| TP + WTConv | DodgerLoopDay       | 0.5                  | 0.15     | 0.021    | 0.143     | 0.037  |

|            |                       |     |       |       |       |       |
|------------|-----------------------|-----|-------|-------|-------|-------|
| TP + WTCnv | DodgerLoopGame        | 0.5 | 0.478 | 0.239 | 0.5   | 0.324 |
| TP + WTCnv | DodgerLoopWeekend     | 0.5 | 0.261 | 0.13  | 0.5   | 0.207 |
| TP + WTCnv | CricketX              | 0.5 | 0.551 | 0.593 | 0.556 | 0.553 |
| TP + WTCnv | CricketY              | 0.5 | 0.582 | 0.596 | 0.58  | 0.584 |
| TP + WTCnv | CricketZ              | 0.5 | 0.59  | 0.606 | 0.592 | 0.585 |
| TP + WTCnv | FreezerRegularTrain   | 0.5 | 0.876 | 0.876 | 0.876 | 0.876 |
| TP + WTCnv | FreezerSmallTrain     | 0.5 | 0.76  | 0.76  | 0.76  | 0.76  |
| TP + WTCnv | UWaveGestureLibraryX  | 0.5 | 0.786 | 0.771 | 0.783 | 0.773 |
| TP + WTCnv | UWaveGestureLibraryY  | 0.5 | 0.716 | 0.712 | 0.717 | 0.71  |
| TP + WTCnv | UWaveGestureLibraryZ  | 0.5 | 0.701 | 0.687 | 0.703 | 0.689 |
| TP + WTCnv | Lightning7            | 0.5 | 0.808 | 0.828 | 0.803 | 0.805 |
| TP + WTCnv | ToeSegmentation2      | 0.5 | 0.831 | 0.741 | 0.832 | 0.767 |
| TP + WTCnv | DiatomSizeReduction   | 0.5 | 0.967 | 0.975 | 0.924 | 0.942 |
| TP + WTCnv | FaceFour              | 0.5 | 0.886 | 0.888 | 0.9   | 0.888 |
| TP + WTCnv | GestureMidAirD1       | 0.5 | 0.038 | 0.001 | 0.038 | 0.003 |
| TP + WTCnv | GestureMidAirD2       | 0.5 | 0.038 | 0.001 | 0.038 | 0.003 |
| TP + WTCnv | GestureMidAirD3       | 0.5 | 0.038 | 0.001 | 0.038 | 0.003 |
| TP + WTCnv | PickupGestureWiimoteZ | 0.5 | 0.1   | 0.01  | 0.1   | 0.018 |
| TP + WTCnv | AllGestureWiimoteX    | 0.5 | 0.1   | 0.01  | 0.1   | 0.018 |
| TP + WTCnv | AllGestureWiimoteY    | 0.5 | 0.1   | 0.01  | 0.1   | 0.018 |
| TP + WTCnv | AllGestureWiimoteZ    | 0.5 | 0.1   | 0.01  | 0.1   | 0.018 |
| TP + WTCnv | ShakeGestureWiimoteZ  | 0.5 | 0.1   | 0.01  | 0.1   | 0.018 |
| TP + WTCnv | Symbols               | 0.5 | 0.939 | 0.948 | 0.937 | 0.94  |



| TP          | Dataset                | Keypoints Percentage | Accuracy | F1 Score | Precision | Recall |
|-------------|------------------------|----------------------|----------|----------|-----------|--------|
| TP + WTConv | Yoga                   | 0.5                  | 0.853    | 0.856    | 0.85      | 0.851  |
| TP + WTConv | OSULeaf                | 0.5                  | 0.769    | 0.789    | 0.773     | 0.769  |
| TP + WTConv | Ham                    | 0.5                  | 0.457    | 0.451    | 0.454     | 0.447  |
| TP + WTConv | Meat                   | 0.5                  | 0.883    | 0.897    | 0.883     | 0.882  |
| TP + WTConv | GesturePebbleZ1        | 0.5                  | 0.163    | 0.027    | 0.167     | 0.047  |
| TP + WTConv | GesturePebbleZ2        | 0.5                  | 0.152    | 0.025    | 0.167     | 0.044  |
| TP + WTConv | Fish                   | 0.5                  | 0.88     | 0.881    | 0.882     | 0.879  |
| TP + WTConv | Beef                   | 0.5                  | 0.7      | 0.774    | 0.7       | 0.71   |
| TP + WTConv | FordA                  | 0.5                  | 0.768    | 0.778    | 0.765     | 0.764  |
| TP + WTConv | FordB                  | 0.5                  | 0.647    | 0.649    | 0.647     | 0.646  |
| TP + WTConv | ShapeletSim            | 0.5                  | 0.617    | 0.64     | 0.617     | 0.6    |
| TP + WTConv | BeetleFly              | 0.5                  | 0.9      | 0.917    | 0.9       | 0.899  |
| TP + WTConv | BirdChicken            | 0.5                  | 0.8      | 0.8      | 0.8       | 0.8    |
| TP + WTConv | Earthquakes            | 0.5                  | 0.691    | 0.558    | 0.547     | 0.548  |
| TP + WTConv | Herring                | 0.5                  | 0.531    | 0.537    | 0.538     | 0.529  |
| TP + WTConv | ShapesAll              | 0.5                  | 0.862    | 0.883    | 0.862     | 0.856  |
| TP + WTConv | OliveOil               | 0.5                  | 0.9      | 0.871    | 0.854     | 0.859  |
| TP + WTConv | Car                    | 0.5                  | 0.767    | 0.767    | 0.762     | 0.762  |
| TP + WTConv | InsectEPGRegularTrain  | 0.5                  | 0.876    | 0.849    | 0.858     | 0.853  |
| TP + WTConv | InsectEPGSmallTrain    | 0.5                  | 0.703    | 0.694    | 0.724     | 0.686  |
| TP + WTConv | Lightning2             | 0.5                  | 0.852    | 0.853    | 0.856     | 0.852  |
| TP + WTConv | Computers              | 0.5                  | 0.664    | 0.664    | 0.664     | 0.664  |
| TP + WTConv | LargeKitchenAppliances | 0.5                  | 0.709    | 0.708    | 0.709     | 0.708  |

|             |                            |     |       |       |       |       |
|-------------|----------------------------|-----|-------|-------|-------|-------|
| TP + WTConv | RefrigerationDevices       | 0.5 | 0.504 | 0.509 | 0.504 | 0.506 |
| TP + WTConv | ScreenType                 | 0.5 | 0.411 | 0.411 | 0.411 | 0.409 |
| TP + WTConv | SmallKitchenAppliances     | 0.5 | 0.6   | 0.605 | 0.6   | 0.594 |
| TP + WTConv | NonInvasiveFetalECGThorax1 | 0.5 | 0.769 | 0.783 | 0.767 | 0.761 |
| TP + WTConv | NonInvasiveFetalECGThorax2 | 0.5 | 0.846 | 0.846 | 0.841 | 0.841 |
| TP + WTConv | Worms                      | 0.5 | 0.61  | 0.667 | 0.552 | 0.578 |
| TP + WTConv | WormsTwoClass              | 0.5 | 0.649 | 0.67  | 0.667 | 0.649 |
