# Supplementary material for: TimePoint: Accelerated Time Series Alignment via Self-Supervised Keypoint and Descriptor Learning
Source: arXiv:2505.23475 source file (2025-05-29)
Supplement: Supplementary file 6 [file datasets_memory_consumption_table.tex]

\begin{table}[ht]
\centering
\begin{tabular}{|c|c|c|c|}
\hline
\textbf{Dataset} & \textbf{Train Size} & \textbf{Test Size} & \textbf{Signal Length} \\
\hline
ChlorineConcentration & 467 & 3,840 & 166 \\
Crop & 7,200 & 16,800 & 46 \\
ECG5000 & 500 & 4,500 & 140 \\
TwoPatterns & 1,000 & 4,000 & 128 \\
UWaveGestureLibraryX & 896 & 3,582 & 315 \\
Wafer & 1,000 & 6,164 & 152 \\
Yoga & 300 & 3,000 & 426 \\
\hline
\end{tabular}
\caption{Datasets train size, test size, and signal length for GPU RAM consumption experiment.}
\label{tab:dataset_characteristics}
\end{table}
